# Supplementary material for: Analytic 3D vector non-uniform Fourier crystal optics in arbitrary $\bar{\bar{\varepsilon}}$ dielectric
Source: arXiv:2412.17224 source file (2025-10-17)
Supplement: Supplementary file 1 [file sn-Supplementary_Notes.pdf]

# Supplementary Notes for: “Analytic 3D vector non-uniform Fourier crystal optics in arbitrary $\bar{\bar{\varepsilon}}$ dielectric”

Chenzhu Xie[1,2,3,4] and Yong Zhang[1,2,3,4*]

[1*]National Laboratory of Solid State Microstructures, Nanjing University, No.15 JinYin Street, Nanjing, 210093, Jiangsu, China.
[2*]College of Engineering and Applied Sciences, Nanjing University, No.163 Xianlin Avenue, Nanjing, 210046, Jiangsu, China.
[3]School of Physics, Nanjing University, No.8 Hankou Road, Nanjing, 210093, Jiangsu, China.
[4]Collaborative Innovation Center of Advanced Microstructures, Nanjing University, No.22 Hankou Road, Nanjing, 210093, Jiangsu, China.

*Corresponding author(s). E-mail(s): zhangyong@nju.edu.cn;
Contributing authors: xczphysics@gmail.com;

# Contents


**1 Supplementary Note 1** **3**

1.1 A top-down revisitation of crystal optics . . . . . . . . . . . . . . . . 3

1.2 Four issues we have identified along the pilgrimage . . . . . . . . . . 5

**2 Supplementary Note 2** **7**

2.1 Bridge the gap from $n^{\omega}(\hat{k}) \in \mathbb{C}_{\mathrm{r}}(\mathbb{R}^2_{\ominus})$ to $k_{\mathrm{z}}^{\omega}(\bar{k}_{\rho}) \in \mathbb{C}_{\mathrm{z}}(\mathbb{R}^2_{\rho})$ . . . . . . . 7

2.2 Eigensystem pairs of non-uniform Fourier crystal optics . . . . . . . . 11

**3 Supplementary Note 3** **13**

3.1 Transformations for vectors between $\mathcal{Z}, \mathcal{C}$ frames . . . . . . . . . . . . 13

3.2 Transformations for vectors between $\curlywedge, \ominus$ coordinates . . . . . . . . . 16

3.3 Conventions and relations for tensors $\bar{\bar{\eta}}^{\omega}, \bar{\bar{\varepsilon}}_{\mathrm{r}}'^{\omega}, \bar{\bar{\bar{\chi}}}_{\omega}^{(2)}$ . . . . . . . . . . . 17

**4 Supplementary Note 4** **20**

4.1 Uniform plane waves in spherical $\mathcal{C}$ frame . . . . . . . . . . . . . . . . 20

4.2 Non-uniform Fourier crystal optics in rectangular $\mathcal{Z}$ frame . . . . . . 23

**5 Supplementary Note 5** **26**

5.1 The transition matrix field constructed by the superimposed electric vector field's spatiotemporal spectrum . . . . . . . . . . . . . . . . . . . 26

# 1 Supplementary Note 1

Through a careful comparison of our detailed treatment to Maxwell equations below and the mathematical strategies in the relevant citations, one can grasp our favored symbols without needing much additional clarification (some necessary information are provided).

## 1.1 A top-down revisitation of crystal optics

By successively substituting the one-dimensional(1D) *Fourier transform*(FT)[1]

$$\bar{\mathit{\Psi}}_z^t(\bar{\rho}) = \mathcal{F}_t\left[\bar{\mathit{\Psi}}_z^\omega\right] := \frac{1}{2\pi}\int_{-\infty}^{+\infty} \bar{\mathit{\Psi}}_z^\omega \cdot \mathbb{e}^{-\mathbb{i}\omega t}\, \mathbb{d}\omega \tag{S1}$$

*1* | *13*.

followed by applying its inverse

$$\mathcal{F}_\omega^{-1}[\cdot] = \int_{-\infty}^{+\infty} \cdot\, \mathbb{e}^{\mathbb{i}\omega t}\, \mathbb{d}t, \tag{S2}$$

*1* | *13*.

and then linearly combining $\bar{E}_\rho^\omega, \bar{H}_\rho^\omega := \left(E_x^\omega,\ E_y^\omega\right)^\intercal, \left(H_x^\omega,\ H_y^\omega\right)^\intercal$ to express $E_z^\omega, H_z^\omega$ from the two curl equations of $\bar{E}^\omega, \bar{H}^\omega = \bar{E}^\omega(\bar{r}), \bar{H}^\omega(\bar{r}) =: \bar{E}_z^\omega(\bar{\rho}), \bar{H}_z^\omega(\bar{\rho}) \in \mathbb{C}^3\left(\mathbb{R}^3\right)$ in the $\omega$ domain, the differential form of Maxwell's equations governing linear and nonlinear crystal optics(LCO & NCO) reduces to a 1st-order(1O), inhomogeneous $4\times4$ matrix differential equation $\partial_z\bar{\mathit{\Psi}}_z^\omega = \mathbb{i}\bar{\bar{A}}_z^\omega\cdot\bar{\mathit{\Psi}}_z^\omega + \bar{B}_z^\omega$ concerning $\bar{\mathit{\Psi}}_z^\omega := \left(\bar{E}_{\rho z}^\omega,\ \bar{H}_{\rho z}^\omega\right)^\intercal$[2–5], possessing an explicit solution $\bar{\mathit{\Psi}}_z^\omega(\bar{\rho}) = \mathbb{e}^{\mathbb{i}\bar{\bar{A}}^\omega z}\cdot(\bar{\mathit{\Psi}}_0^\omega + \int_0^z \mathbb{e}^{-\mathbb{i}\bar{\bar{A}}^\omega s}\cdot\bar{B}_s^\omega\ \mathbb{d}s)$, given that $\bar{\bar{A}}^\omega(\bar{r}) \equiv \bar{\bar{A}}_{[4\times4]}^\omega$ is independent of position $\bar{r}$, that is, the linear part/response of (i.e., the 2nd-order(2O) tensors $\bar{\bar{\varepsilon}}_z^\omega, \bar{\bar{\mu}}_z^\omega; \bar{\bar{\xi}}_z^\omega, \bar{\bar{\zeta}}_z^\omega$[6, 7] in) the constitutive relations(CRs) embedded within $\bar{\bar{A}}_z^\omega(\bar{\rho})$ is uniformly distributed[4, 8] throughout the homogeneous planar slab material, whose front face's inward normal is chosen to be the +z-axis of the three-dimensional(3D) laboratory coordinate system (LCS)[9], also referred to as the $\mathcal{Z}$ frame.

Following the same procedure, plugging the two-dimensional(2D) Fourier integral (namely, the *inverse Fourier transform*(IFT)) of the *spatiotemporal spectrum* $\bar{\psi}_z^\omega(\bar{k}_\rho) := \left(\bar{G}_{\rho z}^\omega,\ \mathcal{F}\left[\bar{H}_{\rho z}^\omega\right]\right)^\intercal$ of $\bar{\mathit{\Psi}}_z^\omega(\bar{\rho})$ (i.e., a superposition of monochromatic plane waves $\bar{\psi}_z^\omega(\bar{k}_\rho)$ along different directions in the *spatial frequency* $\bar{k}_\rho := \left(k_x,\ k_y\right)^\intercal \in \mathbb{R}_\rho^2$ *domain* of the $\mathcal{Z}$ frame):

$$\bar{\mathit{\Psi}}_z^\omega(\bar{\rho}) = \mathcal{F}^{-1}\left[\bar{\psi}_z^\omega\right] := \iint_{-\infty}^{+\infty} \bar{\psi}_z^\omega \cdot \mathbb{e}^{\mathbb{i}\bar{k}_\rho\cdot\bar{\rho}}\, \mathbb{d}k_x\mathbb{d}k_y \tag{S3}$$

*2* | *13*, *28*.

into the above inhomogeneous equation for $\bar{\mathit{\Psi}}_z^\omega(\bar{\rho})$, and performing a 2D FT

$$\mathcal{F}[\cdot] := \frac{1}{(2\pi)^2}\iint_{-\infty}^{+\infty} \cdot\mathbb{e}^{-\mathbb{i}\bar{k}_\rho\cdot\bar{\rho}}\, \mathbb{d}x\mathbb{d}y \tag{S4}$$

*2* | *13*, *28*.

on both sides, one arrives at the equation $\partial_z \bar{\psi}_z^\omega = \mathbb{i}\bar{\bar{a}}^\omega \cdot \bar{\psi}_z^\omega + \bar{b}_z^\omega$ and its solution $\bar{\psi}_z^\omega(\bar{k}_\rho) = \mathbb{e}^{\mathbb{i}\bar{\bar{a}}^\omega z} \cdot (\bar{\psi}_0^\omega + \int_0^z \mathbb{e}^{-\mathbb{i}\bar{\bar{a}}^\omega s} \cdot \bar{b}_s^\omega \, \mathrm{d}s)$ in the *spatiotemporal frequency domain*, where the transitions $\bar{\Psi}_z^\omega(\bar{\rho}), \bar{\bar{A}}^\omega(\partial_{x/y}), \bar{B}_z^\omega(\partial_{x/y}; \bar{\rho}) \rightarrow \bar{\psi}_z^\omega(\bar{k}_\rho), \bar{\bar{a}}^\omega(\bar{k}_\rho), \bar{b}_z^\omega(\bar{k}_\rho)$ are realized.

Linear crystal optics(LCO) then starts with the matrix exponential solution[3, 4, 10, 11] $\bar{\psi}_z^\omega = \mathbb{e}^{\mathbb{i}\bar{\bar{a}}^\omega z} \cdot \bar{\psi}_0^\omega = \sum_{n=0}^{\infty} (\mathbb{i}\bar{\bar{a}}^\omega z)^n \cdot \bar{\psi}_0^\omega / n!$ of the first-order, homogeneous, four-dimensional(4D) differential equation $\partial_z \bar{\psi}_z^\omega = \mathbb{i}\bar{\bar{a}}^\omega \cdot \bar{\psi}_z^\omega$, after discarding the source term $\bar{b}_z^\omega \equiv \bar{0}$ representing the nonlinear optical effects.

The beauty of LCO hides in the potential non-diagonalizability (defectiveness) of the complex anisotropy material-direction $4 \times 4$ matrix $\bar{\bar{a}}^\omega \nRightarrow \overline{\bar{v}_i^{\omega}}^{\mathsf{T}} \cdot \overline{\overline{\lambda_i^{\omega}}}^{\mathsf{T}} \cdot \overline{\bar{v}_i^{\omega}}^{-\mathsf{T}}$, where decomposition $\mathbb{e}^{\mathbb{i}\bar{\bar{a}}^\omega z} = \mathbb{e}^{\mathbb{i}\overline{\bar{v}_i^{\omega}}^{\mathsf{T}} \cdot \overline{\overline{\lambda_i^{\omega}}}^{\mathsf{T}} \cdot \overline{\bar{v}_i^{\omega}}^{-\mathsf{T}} z} = \begin{pmatrix} \bar{v}_1^\omega & \bar{v}_2^\omega & \bar{v}_3^\omega & \bar{v}_4^\omega \end{pmatrix} \cdot \mathbb{e}^{\mathbb{i}\overline{\overline{\lambda_i^{\omega}}}^{\mathsf{T}} z} \cdot \begin{pmatrix} \bar{v}_1^\omega & \bar{v}_2^\omega & \bar{v}_3^\omega & \bar{v}_4^\omega \end{pmatrix}^{-1} = \overline{\bar{v}_i^{\omega}}^{\mathsf{T}} \cdot \overline{\overline{\mathbb{e}^{\mathbb{i}\lambda_i^\omega z}}} \cdot \overline{\bar{v}_i^{\omega}}^{-\mathsf{T}}$ may not always hold, making numerical solutions to the matrix exponential $\mathbb{e}^{\mathbb{i}\bar{\bar{a}}^\omega z}$ necessary under specific $\{\bar{k}_\rho, \omega; \bar{\bar{\varepsilon}}^\omega, \bar{\bar{\mu}}^\omega, \bar{\bar{\xi}}^\omega, \bar{\bar{\zeta}}^\omega\}$ combinations[12]. The unfolding of 2-, 3-, and 4-fold (algebraic $d_j\{\lambda_i^\omega\} \geq$ geometric $m_j\{\bar{v}_i^\omega\}$) degeneracies/multiplicities has sparked profound investigations into singular optics[13, 14], EPs[15] in various non-Hermitian systems[16], and inhomogeneous eigensubwaves exhibiting linear, quadratic, and cubic coordinate-dependent amplitude behaviors[17, 18].

The last insight capturing the polynomial $z$ dependence of eigen-amplitudes in the first, second, and third orders can be mathematically understood/derived through Jordan-Chevalley decomposition $\bar{\bar{J}}^\omega = \overline{\overline{\lambda_i^{\omega}}}^{\mathsf{T}} + \bar{\bar{N}}^\omega$ from Jordan normal form of $\bar{\bar{a}}^\omega = \overline{\bar{v}_i^{\omega}}^{\mathsf{T}} \cdot \bar{\bar{J}}^\omega \cdot \overline{\bar{v}_i^{\omega}}^{-\mathsf{T}}$, leading to the ultimate expansion for the *transition matrix* $\mathbb{e}^{\mathbb{i}\bar{\bar{a}}^\omega z} = \overline{\bar{v}_i^{\omega}}^{\mathsf{T}} \cdot \overline{\overline{\mathbb{e}^{\mathbb{i}\lambda_i^\omega z}}} \cdot \sum_{n=0}^{3} (\mathbb{i}\bar{\bar{N}}^\omega z)^n / n! \cdot \overline{\bar{v}_i^{\omega}}^{-\mathsf{T}}$[17], where $\overline{\bar{v}_i^{\omega}}^{\mathsf{T}}$ contains the generalized eigenvectors $\{\bar{v}_i^\omega\}_j$ corresponding to the degenerate eigenvalues $\{\lambda_i^\omega\}_j$, with $\bar{\bar{N}}^\omega$ being a nilpotent matrix of order 4, whose powers $\bar{\bar{N}}_\omega^0, \bar{\bar{N}}_\omega^1, \bar{\bar{N}}_\omega^2, \bar{\bar{N}}_\omega^3$ generate $z^0, z^1, z^2, z^3$ dependence of *basis coefficients* $\{\bar{\bar{N}}_\omega^n \cdot \overline{\bar{v}_i^{\omega}}^{-\mathsf{T}} \cdot \bar{\psi}_0^\omega\}$ (or equivalently, *polarization states* $\{\overline{\bar{v}_i^{\omega}}^{\mathsf{T}} \cdot \bar{\bar{N}}_\omega^n\}$) respectively, expecting associated eigenvalues $\lambda_i^\omega(n)$ possess positive imaginary parts to guarantee eventual absorption[15, 18–20] along +z, marking the farthest reaches of LCO.

The 1O-4D equation $\partial_z \bar{\psi}_z^\omega = \mathbb{i}\bar{\bar{a}}_{[4\times4]}^\omega \cdot \bar{\psi}_z^\omega$ can be further reduced to a 2O-2D pure electric field wave equation $(\bar{\bar{c}}^\omega \cdot \partial_z^2 - \bar{\bar{d}}^\omega \cdot \partial_z - \bar{\bar{e}}^\omega \cdot)\bar{G}_{\rho z}^\omega = \bar{0}_{[2\times1]}$[18], by eliminating $\mathcal{F}\left[\bar{H}_{\rho z}^\omega\right]$ in $\bar{\psi}_z^\omega$[20]. Inserting the trial solution $\bar{G}_{\rho z}^\omega = \mathbb{e}^{\mathbb{i}\bar{\bar{k}}_{\mathrm{z}[2\times2]}^\omega z} \cdot \bar{E}_{\rho 0}^\omega$ yields a difficult system of 4 coupled equations $\bar{\bar{c}}^\omega \cdot \bar{\bar{k}}_{\omega \mathrm{z}}^2 + \mathbb{i}\bar{\bar{d}}^\omega \cdot \bar{\bar{k}}_{\mathrm{z}}^\omega + \bar{\bar{e}}^\omega = \bar{\bar{0}}_{[2\times1]}$[18] regarding $\bar{\bar{k}}_{\mathrm{z}[2\times2]}^\omega$. The additional degrees of freedom provided by the $2 \times 2$ tensor (field) $\bar{\bar{k}}_{\mathrm{z}}^\omega(\bar{k}_\rho)$ can also be employed to break the degeneracy of eigenvectors along multiple singularity directions $\{\bar{k}_{\rho i}\}$ in $\bar{k}_\rho$ domain, similar to how $\bar{\bar{a}}_{[4\times4]}^\omega$ functions.

If we further reduce the dimensionality of the "z component of the wave vector" $\bar{\bar{a}}_{[4\times4]}^\omega$[4, 10]($\rightarrow \bar{\bar{k}}_{\mathrm{z}[3\times3]}^\omega$[7, 17, 18]) $\rightarrow \bar{\bar{k}}_{\mathrm{z}[2\times2]}^\omega$[18]$\rightarrow k_{\mathrm{z}}^\omega$[1] from tensors to scalar, the contracted solution space will exclude the sub-eigenvectors to the extent that their degeneracy can no longer be resolved, leaving only correct eigenvalue(s) preserved in $k_{\mathrm{z}}^\omega$ determined by $\det(\bar{\bar{a}}_{[4\times4]}^\omega - k_{\mathrm{z}}^\omega \bar{\bar{\mathrm{I}}})$[5, 10, 17]$= \det[k_{0\omega}^2 \bar{\bar{\varepsilon}}_{[3\times3]}^\omega + (\bar{\bar{k}}_\omega^\times + k_0^\omega \bar{\bar{\xi}}^\omega)\bar{\bar{\mu}}_\omega^{-1}(\bar{\bar{k}}_\omega^\times - k_0^\omega \bar{\bar{\zeta}}^\omega)]$[1, 7, 21–24]$= \det(k_{\omega \mathrm{z}}^2 \bar{\bar{c}}^\omega + \mathbb{i}k_{\mathrm{z}}^\omega \bar{\bar{d}}^\omega + \bar{\bar{e}}_{[2\times2]}^\omega)$[5, 25]$= 0$, which can then be

substituted into the nullspace[7, 24] (whose dimension might exceed 1?[10]) of the corresponding 4D/3D/2D homogeneous system to obtain the associated eigenvector(s). Specifically, for non-homogeneous system $\bar{\bar{a}}^{\omega} \cdot \bar{\psi}_z^{\omega} = k_z^{\omega} \bar{\psi}_z^{\omega}$ (with an odd spectrum[14] $k_z^{\omega}$), eigenstructure of $\bar{\bar{a}}^{\omega}$ can also be numerically obtained[26] through Schur factorization or QR decomposition. However, due to the inherent one-to-one correspondence between eigenvalues and eigenvectors originated from the scalar (field) nature of $k_z^{\omega}(\bar{k}_\rho) \in \mathbb{C}_z(\mathbb{R}_\rho^2)$, once eigenvalues degenerate (normal), eigenvectors can no longer be resolved (abnormal), leaving an EP in that direction.

Other methods that ultimately form eigenvalue problems[27–29] — thereby potentially yielding explicit solutions, particularly for eigenvectors — either involve the use of zero-divergence postulate(s) (though not essential[30]), which results in eigenvalues $n^{\omega}(\hat{k}) \in \mathbb{C}_r(\mathbb{R}_\ominus^2)$ being functions of real direction[12–14, 31] $\hat{k} \in \mathbb{R}_\ominus^2$ rather than real spatial frequency $\bar{k}_\rho \in \mathbb{R}_\rho^2$, thus failing to meet the requirements of standard FT and phase continuity boundary conditions in dissipative/active case[32–34]; or require that the constitutive matrix can be (unitarily/Schur) diagonalized[9, 35, 36], which holds true only for normal matrices ((anti-)symmetric or (anti-)Hermitian), but not for arbitrary $\bar{\bar{\varepsilon}}^{\omega}, \bar{\bar{\mu}}^{\omega}, \bar{\bar{\xi}}^{\omega}, \bar{\bar{\zeta}}^{\omega}$ tensors.

Across all models where either the scalar field $n^{\omega}(\hat{k})$ ('s $(\cdot)^{-1}$ or $(\cdot)^{-2}$) or $k_z^{\omega}(\bar{k}_\rho)$ serves as the eigenvalue $\lambda^{\omega}$, EPs are generally unavoidable and do not "automatically self-reveal" their internal structure. — Moreover, when it comes to obtaining eigenvalues, all models[1, 23, 28] that choose $k_z^{\omega}(\bar{k}_\rho) \in \mathbb{C}_z(\mathbb{R}_\rho^2)$ as the eigenvalue, in the broadest sense, invariably necessitate the numerical solution of Booker quartic[5, 7, 37–39] concerning $k_z^{\omega}$ even in the absence of both the Faraday effect and bianisotropic coupling, though this is procedurally justified for experimental consistency (meeting the requirements of FT and phase continuity). In contrast, models[9, 12, 13, 20, 22, 27, 31, 35] that take $n^{\omega}(\hat{k}) \in \mathbb{C}_r(\mathbb{R}_\ominus^2)$ as the eigenvalue, while easily deriving closed-form solution from bi-quadratic equation = even spectrum[13, 14] regarding $n^{\omega}$ (in the case of Lorentz-reciprocity = no Faraday effect[14, 21, 30] or non-magnetoelectric = no bianisotropic coupling[7, 14]), neither fit within the FT framework nor satisfy the in-plane momentum conservation when energy transfer occurs between light and matter, thus aligning less well with experimental applications where eigenwaves of the slab material are often excited from air[18].

Clearly, there is a gap that needs to be bridged between the two: how can the closed-form solution $n^{\omega}(\hat{k}) \in \mathbb{C}_r(\mathbb{R}_\ominus^2)$ of the bi-quadratic characteristic equation be modified to more align with the formally and experimentally correct numerical solution $k_z^{\omega}(\bar{k}_\rho) \in \mathbb{C}_z(\mathbb{R}_\rho^2)$ of the quartic equation? To tackle this issue, this paper demonstrates by standardizing the $3 \times 2$ transition matrix of M.V. Berry's 2003 model and extending M.V. Berry's uniform plane waves in purely electrically anisotropic unbounded media[13] to non-uniform[18, 32, 33] Fourier[1] crystal optics(FCO).

## 1.2 Four issues we have identified along the pilgrimage

Both quantum mechanics and the wave optics that gave birth to it, present their plane wave solutions in the form of matrix exponentials in the broadest sense. As the ultimate frontier of understanding and computation, the perfect solution to the matrix

exponential of defect matrices corresponding to non-Hermitian systems remains an eternal shared pursuit across mathematics, physics, and computer science[11].

1) Concerning wave optics in materials with bi-anisotropy, — as an exact solution to the first-order, homogeneous, four-dimensional(4D) differential equation $\partial_z \bar{\psi}_z^\omega = \mathbb{i}\bar{\bar{a}}_{[4\times4]}^\omega \cdot \bar{\psi}_z^\omega$, the matrix exponential solution $\bar{\psi}_z^\omega = \mathbb{e}^{\mathbb{i}\bar{\bar{a}}^\omega z} \cdot \bar{\psi}_0^\omega$[3, 4, 10, 11] with Jordan decomposition(JD) for constitutive matrix $\bar{\bar{a}}^\omega = \overline{\bar{v}_i^\omega}^\mathsf{T} \cdot (\bar{\bar{N}}^\omega + \overline{\bar{\lambda}_i^\omega}^\mathsf{T}) \cdot \overline{\bar{v}_i^\omega}^{-\mathsf{T}}$ can theoretically unfold the degenerate polarization states, i.e., generalized subeigenvectors $\bar{v}_i^\omega$, of the electromagnetic field's spatiotemporal spectrum $\bar{\psi}_z^\omega(\bar{k}_\rho) := \left(\bar{G}_{\rho z}^\omega,\ \mathcal{F}\left[\bar{H}_{\rho z}^\omega\right]\right)^\mathsf{T}$ at exceptional points(EPs), also known as optical singularities[13, 14] — if not addressed, resulting in unphysical infinite transmittance when applying boundary conditions afterwards. Yet, in practice, for matrix field $\bar{\bar{a}}^\omega(\bar{k}_\rho)$ across all spatial frequencies $\bar{k}_\rho$, JD can only be performed numerically and proves unstable near EPs[11].

2) Alternatively, using QR/Schur factorization or solving quartic equations through root-finding algorithms/formulas[10] or Newton's iteration to obtain the four eigenvalues $\lambda_i^\omega$, and subsequently determining the polarization states to construct[10, 22, 23] the $4 \times 4$ transition matrix $\bar{\bar{a}}^\omega \overset{?}{=} \overline{\bar{v}_i^\omega}^\mathsf{T} \cdot \overline{\bar{\lambda}_i^\omega}^\mathsf{T} \cdot \overline{\bar{v}_i^\omega}^{-\mathsf{T}}$, or directly computing the matrix exponential without attaining its eigensystem[3], although numerically well-established[11], encounters issues: for non-Hermitian matrices and long propagation distances, the exponential $\mathbb{e}^{\mathbb{i}\bar{\bar{a}}^\omega z}$ will inevitably diverge, regardless of whether or how $\bar{\bar{a}}^\omega$ is decomposed (even via JD). — This is because all $4\times4$ matrix techniques force the four eigensystems to propagate together $\mathbb{e}^{\mathbb{i}\bar{\bar{a}}^\omega z} = \overline{\bar{v}_i^\omega}^\mathsf{T} \cdot \sum_{n=0}^{3} (\mathbb{i}\bar{\bar{N}}^\omega z)^n / n! \cdot \overline{\overline{\mathbb{e}^{\mathbb{i}\lambda_i^\omega z}}} \cdot \overline{\bar{v}_i^\omega}^{-\mathsf{T}} \overset{?}{=} \overline{\bar{v}_i^\omega}^\mathsf{T} \cdot \overline{\overline{\mathbb{e}^{\mathbb{i}\lambda_i^\omega z}}} \cdot \overline{\bar{v}_i^\omega}^{-\mathsf{T}}$ as a unified $4\times4$ matrix $\bar{\bar{a}}^\omega$ with a shared $z$-value, where eigenvalues of certain backward-propagating eigenwaves will have negative imaginary parts even within absorbing/dissipative media, leading to gain[10] as $z$ increases.

3) After using linear algebra techniques (JD, QR, or solving quartic) to decompose and obtain four eigensystems, one may also choose not to form a unified $4 \times 4$ matrix. Instead, one can further differentiate between forward and backward traveling waves along the +z-direction (which are not necessarily paired, and distinguished by $\mathrm{Re}\,[s_\mathrm{z}^\omega]$ rather than $\mathrm{Re}\,[k_\mathrm{z}^\omega]$, whose values may also include multiple zeros) and separate them to independently calculate the transmission and reflection at the front or rear surfaces, treating it as a semi-infinite medium problem.

If the decomposition is not carried out using JD or an equivalent technique[17, 18] to attain $n^\omega(\hat{k})$[9, 12–14, 20, 22, 27, 29, 31, 35] or $k_\mathrm{z}^\omega(\bar{k}_\rho)$[1, 5, 7, 23, 28, 37–39] as the eigenvalue $\lambda^\omega$, and if these eigenvalues are not retained with their corresponding ground true eigenvectors $\bar{v}^\omega$ within the tensor field propagator $\bar{\bar{a}}_{[4\times4]}^\omega$[4, 10],$\bar{\bar{k}}_{\mathrm{z}[3\times3]}^\omega$[7, 17, 18] or $\bar{\bar{k}}_{\mathrm{z}[2\times2]}^\omega$[18], then EPs will no longer be resolved, irrespective of whether the eigensystems are arranged into a $4 \times 4$ matrix or matrices of other sizes.

4) Owing to the low symmetry of both crystal classes and the *3D Cartesian/rectangular coordinate system* ($\curlywedge$), which leads to the coupling $k_\mathrm{z}^\omega = f(\bar{k}_\rho, k_\mathrm{z}^\omega)$ between independent/input and dependent/output variables $\bar{k}_\rho \leftrightarrow k_\mathrm{z}^\omega$, all models[1, 23, 28] taking $k_\mathrm{z}^\omega(\bar{k}_\rho) \in \mathbb{C}_\mathrm{z}(\mathbb{R}_\rho^2)$ as the eigenvalue generally[7, 24] require a numerical solution equivalent to Booker quartic[5, 7, 37–39] regarding $k_\mathrm{z}^\omega$, even in the absence of both the Faraday effect[14, 30] and bi-anisotropic coupling[14]. — Whereas, in such cases,

all models choosing $n^\omega(\hat{k}) \in \mathbb{C}_\mathrm{r}(\mathbb{R}^2_\ominus)$ in real *spherical coordinate systems* ($\ominus$) as the eigenvalue $\lambda^\omega$, always possess closed-form solution from bi-quadratic equation[21] = even spectrum[13, 14] concerning $n^\omega$.

Nevertheless, from the standpoint of experimental/boundary conditions and logical/formal correctness, one must opt for $k_\mathrm{z}^\omega(\bar{k}_\rho)$ rather than $n^\omega(\hat{k})$: Since the eigenwaves within the commonly used slab materials in experiments are often excited from the air, the physical condition of phase continuity at the front and rear surfaces of the plate, combined with the mathematical definition of the Fourier transform, jointly require that the independent variable for monochromatic plane waves be the rectangular transverse spatial frequency $\bar{k}_\rho \in \mathbb{R}^2_\rho$ rather than the sperical radial directional *real unit vector* $\hat{k} \in \mathbb{R}^2_\ominus$.

The contradiction presented in the last(4th) point introduces the core mission of this work: in terms of eigenvalue $\lambda^\omega$, how to transition from $\hat{k} \in \mathbb{R}^2_\ominus$ to $\bar{k}_\rho \in \mathbb{R}^2_\rho$ as its dependent variable, while converting from the closed-form solution $n^\omega \in \mathbb{C}_\mathrm{r}$ to the numerical solution $k_\mathrm{z}^\omega \in \mathbb{C}_\mathrm{z}$ as its independent variable, especially in the case of Lorentz-reciprocity = no Faraday effect[14, 21, 30] or non-magnetoelectric = no bi-anisotropic coupling[7, 13, 14], where $n^\omega \in \mathbb{C}_\mathrm{r}$ preserves its closed form from bi-quadratic. — This enables us to maintain the analytic advantage (potentially faster and more physical) while better aligning with boundary conditions (formally/experimentally more correct thus accurate).

For illustration, we showcase the path to bridge this gap by standardizing the $3 \times 2$ transition matrix of M.V. Berry's 2003 model and extending Berry's uniform plane waves in purely electrically anisotropic unbounded media[13] to non-uniform[18, 32, 33] FCO[1], in light of the analytical benefits conferred by the eigenvalue problem, and without further restricting the $\bar{\bar{\varepsilon}}^\omega$ tensor. Additionally, Berry naturally offers eigenvectors in the dielectric *principal coordinate system* (PCS), positioning Berry's model as a ideal cornerstone for nonlinear[40, 41] Fourier crystal optics(NFCO).

Notably, this approach ensures maximum compatibility with existing models, including numerous others[12, 29, 31] where direction $\hat{k} \in \mathbb{R}^2_\ominus$ is used as an independent variable (even if they[9, 20, 22, 27, 35] do not involve the divergence equation), while providing 'patching' guidance for the eigenvalues $n^\omega \in \mathbb{C}_\mathrm{r} \to k_\mathrm{z}^\omega \in \mathbb{C}_\mathrm{z}$ and their independent variables $\hat{k} \in \mathbb{R}^2_\ominus \to \bar{k}_\rho \in \mathbb{R}^2_\rho$ with zero alteration to the cores of the current models, facilitating seamless installation of our provided plugins as extensions.

Quoted @ *1* p. *26*.

# 2 Supplementary Note 2

## 2.1 Bridge the gap from $n^\omega(\hat{k}) \in \mathbb{C}_\mathrm{r}(\mathbb{R}^2_\ominus)$ to $k_\mathrm{z}^\omega(\bar{k}_\rho) \in \mathbb{C}_\mathrm{z}(\mathbb{R}^2_\rho)$

In a natural rest Cartesian frame, the wave equations for vector electric field $\bar{E}_z^t(\bar{\rho}) := \bar{E}(\bar{r}, t)$, its *temporal spectrum* $\bar{E}_z^\omega(\bar{\rho})$, and its spatiotemporal spectrum $\bar{G}_z^\omega(\bar{k}_\rho) := \bar{g}^\omega \cdot e^{\mathrm{i} k_\mathrm{z}^\omega z}$, propagating in a potentially electrical anisotropic nonmagnetic medium are

given by:

$$\nabla \times \left(\nabla \times \bar{E}_z^t\right) + \mu_0 \left(\bar{\bar{\varepsilon}}_z^t \,\tilde{*}\, \frac{\partial^2}{\partial t^2} + \bar{\bar{\sigma}}_z^t \,\tilde{*}\, \frac{\partial}{\partial t}\right) \bar{E}_z^t = \bar{0}, \tag{S5a}$$

$$\nabla \left(\nabla \cdot \bar{E}_z^\omega\right) - \nabla^2 \bar{E}_z^\omega - k_{0\omega}^2 \bar{\bar{\varepsilon}}'^{\omega}_{\mathrm{rz}} \cdot \bar{E}_z^\omega = \bar{0}, \tag{S5b}$$

1 | 26.

$$\left(k_\omega^2 - \bar{k}^\omega \bar{k}_\omega^\intercal - k_{0\omega}^2 \bar{\bar{\varepsilon}}'^{\omega}_{\mathrm{rz}}\right) \cdot \bar{g}^\omega = \bar{0}, \tag{S5c}$$

3 | 8, 10, 11.

with the help of Eqs. (S1) to (S4) and under the condition of Eq. (1) in the main text, where magnetic permeability, electric permittivity, and conductivity tensors are defined as $\bar{\bar{\mu}} := \mu_0 \bar{\bar{\mu}}_{\mathrm{r}}, \bar{\bar{\varepsilon}} := \varepsilon_0 \bar{\bar{\varepsilon}}_{\mathrm{r}}, \bar{\bar{\sigma}}$ (characterized by two overhead short bars $^=$ indicating that they are second-order tensors) with the vacuum permeability $\mu_0$, the vacuum permittivity $\varepsilon_0$ and the identity tensor $\bar{\bar{\mu}}_{\mathrm{r}} \equiv \bar{\bar{\mathrm{I}}}_{(3\times3)}$ for naturally occurring optical materials. For convenience, we define $\bar{E}_z^t(\bar{\rho}), \bar{\bar{\varepsilon}}_z^t(\bar{\rho}), \bar{\bar{\sigma}}_z^t(\bar{\rho}) := \bar{E}(\bar{r}, t), \bar{\bar{\varepsilon}}(\bar{r}, t), \bar{\bar{\sigma}}(\bar{r}, t)$ as functions of the propagation distance $z$ and time $t$ (usually, physical quantities with a subscript $z$ are also functions of $x, y$ or transverse spatial frequency $k_{\mathrm{x}}, k_{\mathrm{y}}$) and $\nabla, \bar{E}, \bar{r}, \bar{\rho}, \bar{0} := \left(\partial/\partial x,\, \partial/\partial y,\, \partial/\partial z\right)^\intercal, \left(E_{\mathrm{x}},\, E_{\mathrm{y}},\, E_{\mathrm{z}}\right)^\intercal, \left(x,\, y,\, z\right)^\intercal, \left(x,\, y\right)^\intercal, \left(0,\, 0,\, 0\right)^\intercal$ as column vectors (characterized by one single short bar $^-$ overhead, except for $\nabla$) in the rectangular coordinate system ($\curlywedge$), which do not include the corresponding unit base vectors $\hat{\mathrm{e}}_{\mathrm{x}}, \hat{\mathrm{e}}_{\mathrm{y}}, \hat{\mathrm{e}}_{\mathrm{z}}$ (where the hat $\hat{}$ represents the unit column vector, combined with the upright 'e' to form the unit base vector $\hat{\mathrm{e}}$, whose direction is generally fixed). The outer/cross/vector product $\times$ maintains its original definition, e.g., $\nabla \times \bar{E} = \left(\partial E_{\mathrm{z}}/\partial y - \partial E_{\mathrm{y}}/\partial z,\, \partial E_{\mathrm{x}}/\partial z - \partial E_{\mathrm{z}}/\partial x,\, \partial E_{\mathrm{y}}/\partial x - \partial E_{\mathrm{x}}/\partial y\right)^\intercal$. We chanced upon the observation that our notational choices for vectors and tensors (both single and multiple overlines) closely resemble the conventions employed by Professor T.G. Mackay (single and multiple underlines)[30, 42], whereas the underlines in this article serve a different role.

Besides, a strict distinction is made between *upright/regular/roman/normal* and *italicized/oblique* mathematical fonts in this paper. *Italics/Obliques* are exclusively used to denote *continuous variables* such as the body $E$ of $E_{\mathrm{z}}$, while all other physical quantities (including discrete variables) and symbols are represented in upright fonts such as the body $\mu$ and the subscript r, z of $\bar{\bar{\mu}}_{\mathrm{r}}, E_{\mathrm{z}}$. Consequently, x, y, z in upright font signify directions, different from the italicized spatial coordinates $x, y, z$. Additionally, the operator $\tilde{*}$ denotes convolution in the time $t$ domain or the angular/temporal frequency $\omega$ domain, distinguished from the convolution operator $*$ in the spatial $x, y$ domain or the spatial frequency $k_{\mathrm{x}}, k_{\mathrm{y}}$ domain. Moreover, we emphasize the $\omega$ dispersion of the dielectric tensor $\bar{\bar{\varepsilon}}'^{\omega}_{\mathrm{rz}} := \bar{\bar{\varepsilon}}^{\omega}_{\mathrm{rz}} + \frac{\mathrm{i}}{\varepsilon_0 \omega} \bar{\bar{\sigma}}_z^\omega$, the temporal spectrum of the vector electric field $\bar{E}_z^\omega$, and the vacuum wavenumber $k_0^\omega := \omega/\mathrm{c}$ in which the speed of light $c = 1/\sqrt{\mu_0 \varepsilon_0}$.

Upon integration with the divergence equation, Eq. (S5c) can 'formally' continue to be expressed as

$$\left(1 - \hat{k}^\omega \hat{k}^\omega - \frac{\bar{\bar{\varepsilon}}'^{\omega}_{\mathrm{r}}}{n_\omega^2}\right) \cdot \bar{g}^\omega = \bar{0}, \tag{S6a}$$

2 | 10, 11.

$$\hat{k}^\omega \cdot \bar{\bar{\varepsilon}}^{\omega}_{\mathrm{r}} \cdot \bar{g}^\omega = 0, \tag{S6b}$$

where a non-unit bi-directional complex vector $\hat{k}^\omega$ and the 'formally' defined refractive index $n^\omega$ are employed as intermediate physical quantities:

$$\hat{k}^\omega := \bar{k}^\omega / k^\omega, \tag{S7a}$$

$$\neq \bar{k}^\omega / |\bar{k}^\omega| =: \bar{k} / \sqrt{\bar{k} \cdot \bar{k}^*} =: \mathcal{N}\left[\bar{k}^\omega\right], \tag{S7b}$$

$$n^\omega := k^\omega / k_0^\omega, \tag{S7c}$$

in which

$$\bar{k}^\omega := \left(k_\mathrm{x},\, k_\mathrm{y},\, k_\mathrm{z}^\omega\right)^\mathsf{T}, \tag{S8a}$$

$$k^\omega := \sqrt{k_\omega^2} := \sqrt{k_\rho^2 + k_{\mathrm{z}\omega}^2} \tag{S8b}$$

$$\neq |\bar{k}^\omega| = \sqrt{k_\rho^2 + |k_\mathrm{z}^\omega|^2} = \sqrt{|\bar{k}_\mathrm{R}^\omega|^2 + k_{\omega\mathrm{I}}^2}, \tag{S8c}$$

$$k_\mathrm{z}^\omega := \sqrt{k_\omega^2 - k_\rho^2} \tag{S8d}$$ *3* | *12*, *23*, *23*.

$$= \sqrt{k_{0\omega}^2 n_\omega^2 - k_\rho^2} = k_0^\omega \sqrt{n_\omega^2 - NA_{0\omega}^2}, \tag{S8e}$$

where $NA_0^\omega := k_\rho / k_0^\omega$ representing the numerical aperture (N.A.) in the air, is a function of $\bar{k}_\rho$ as well.

Rewriting Eq. (S6) in the context of the non-diffractive portion $\bar{d}^\omega := \bar{\bar{\varepsilon}}_\mathrm{r}^{\prime\omega} \cdot \bar{g}^\omega$ of the spatiotemporal spectrum of the electric displacement vector $\bar{D}_z^\omega$ yields the characteristic equation of the $3 \times 3$ characteristic matrix $\bar{\bar{M}}_\curlywedge^\omega := \left(1 - \hat{k}^\omega \hat{k}^\omega\right) \cdot \bar{\bar{\eta}}^\omega$ under lateral constraints:

$$\left(1 - \hat{k}^\omega \hat{k}^\omega\right) \cdot \bar{\bar{\eta}}^\omega \cdot \bar{d}^\omega = \frac{1}{n_\omega^2} \bar{d}^\omega, \tag{S9a}$$ *2* | *10*, *11*.

$$\hat{k}^\omega \cdot \bar{d}^\omega = 0, \tag{S9b}$$

where the complex reciprocal relative dielectric tensor $\bar{\bar{\eta}}^\omega := \bar{\bar{\varepsilon}}_{\mathrm{r}\omega}^{\prime -1}$.

To obtain a uniform plane wave $\bar{d}^{\prime\omega} \cdot \mathbb{e}^{\mathbb{i} k^{\prime\omega}(\hat{k}) \hat{k} \cdot \bar{r}}$ in any real direction $\hat{k}$ (rather than bi-directional $\hat{k}^\omega$ in Eq. (S9)) within a $4\pi$ solid angle allowed by Maxwell's equations in a pure electrically anisotropic homogeneous unbounded medium, Berry[13] took an alternative form of Eq. (S9) that comes from substituting $\bar{E}_z^\omega = \bar{g}^{\prime\omega} \cdot \mathbb{e}^{\mathbb{i} k^{\prime\omega}(\hat{k}) \hat{k} \cdot \bar{r}}$ instead of $\bar{E}_z^\omega = \bar{g}^\omega \cdot \mathbb{e}^{\mathbb{i}\left[\bar{k}_\rho \cdot \bar{\rho} + k_z^\omega(\bar{k}_\rho) \cdot z\right]}$ into Eq. (S5):

$$\left(1 - \hat{k}\hat{k}\right) \cdot \bar{\bar{\eta}}^\omega \cdot \bar{d}^{\prime\omega} = \frac{1}{n_{\prime\omega}^2} \bar{d}^{\prime\omega}, \tag{S10a}$$

$$\hat{k} \cdot \bar{d}^{\prime\omega} = 0, \tag{S10b}$$

where $\hat{k}, n^{\prime\omega}, \bar{g}^{\prime\omega}, \bar{d}^{\prime\omega}$ are updated from $\hat{k}^\omega, n^\omega, \bar{g}^\omega, \bar{d}^\omega$, while $\bar{\bar{\eta}}^\omega$ and the equation's format remain consistent.

Since $\hat{k}$ and $\bar{k}_\rho$ are essentially unrelated, the solutions of Eq. (S10) are not synonymous with the solutions of Eq. (S9), demonstrating that $k^\omega, n^\omega, \bar{g}^\omega, \bar{d}^\omega \neq k'^\omega, n'^\omega, \bar{g}'^\omega, \bar{d}'^\omega$. Moreover, the solving technique for Eq. (S10) cannot be directly employed for solving Eq. (S9), because $\hat{k}^\omega$ is a complex bidirectional vector, unlike the real vector $\hat{k}$. Nevertheless, we have found that, under particular circumstances, the solutions to both of these Eqs. (S9) and (S10) are mathematically linked in their expressions and numerically close.

Drawing inspiration from Brenier[31], we establish the following correlation between Berry's uniform complex wave vector $\bar{k}'^\omega(\hat{k}) := k'^\omega(\hat{k})\hat{k} := k_0^\omega n'^\omega(\hat{k})\hat{k} \in \mathbb{C}_r\left(\mathbb{R}^2_\ominus\right) \times \mathbb{R}^2_\ominus$[13] for Eq. (S10) and non-uniform complex wave vector $\bar{k}^\omega\left(\bar{k}_\rho\right) := \bar{k}_\perp\left(\bar{k}_\rho\right) + \bar{k}^\omega_z\left(\bar{k}_\rho\right) =: k^\omega(\bar{k}_\rho)\hat{k}^\omega(\bar{k}_\rho) := k_0^\omega n^\omega(\bar{k}_\rho)\hat{k}^\omega(\bar{k}_\rho) \in \mathbb{R}^2_\perp\left(\mathbb{R}^2_\rho\right) + \mathbb{C}_Z\left(\mathbb{R}^2_\rho\right)$[1] for Eq. (S9):

$$\text{input real direction } \ \hat{k} = \hat{k}^\omega_R\left(\bar{k}_\rho\right) \ \text{ to obtain uniform } k'^\omega(\hat{k}), \tag{S11a}$$

7 | *10, 10, 11, 11, 12, 23, 24.*

$$\text{output non-uniform } \ k^2_\omega = k^2_{\prime\omega}(\hat{k}) \ \text{ as a function of uniform } k'^\omega(\hat{k}), \tag{S11b}$$

5 | *10, 11, 11, 11, 23.*

where Berry's input variable $\hat{k} = \hat{k}^\omega_R := \mathcal{N}\left\{\mathrm{Re}\left[\bar{k}^\omega\right]\right\} = \mathcal{N}\left\{\mathrm{Re}\left[\left(k_x,\, k_y,\, k^\omega_z\right)^\intercal\right]\right\} = \mathcal{N}\left\{\mathrm{Re}\left[\left(k_x,\, k_y,\, \sqrt{k^2_\omega - k^2_\rho}\right)^\intercal\right]\right\}$ in Eq. (S11a), similar to but different from that of Brenier's, i.e. $\hat{k} = \hat{k}'^\omega_R := \mathcal{N}\left\{\mathrm{Re}\left[\bar{k}'^\omega\right]\right\}$, is set to be a function of the needed output variable $k^2_\omega$ which is further set equal to Berry's output variable $k^2_{\prime\omega}(\hat{k})$, indicating these two Eqs. (S11a) and (S11b) are mutually coupled, leading to the iterative determination of two directions $\hat{k}^\pm$ for each $\bar{k}_\rho$, corresponding to two of Berry's $\pm$ eigenvalue-eigenvector pairs $k^2_{\prime\omega}(\hat{k}), \bar{d}'^\omega(\hat{k})$ which generally do not share the same $\hat{k}$ but always share the same $\bar{k}_\rho$ after modification, as the origin of (wave-vector) birefringence, and as a result of the symmetry breaking of coordinate system (CS)[24].

It's noteworthy that $k^2_\omega$ is not derived from Eqs. (S5c), (S6a) and (S9a) as a function of $\bar{k}_\rho$, but is set directly to match two of Berry's eigenvalues $k^2_{\prime\omega}(\hat{k})$, whose input variables $\hat{k}^+, \hat{k}^-$ corresponding to the same $\bar{k}_\rho$ are usually distinct from each other, where $\pm$ denotes Berry's two modes[13]. The two eigenvalue-eigenvector pairs $k^2_{\prime\omega}(\hat{k}(\bar{k}_\rho, k^2_{\prime\omega})), \bar{d}'^\omega(\hat{k}(\bar{k}_\rho, k^2_{\prime\omega}))$ for the same $\bar{k}_\rho$ determined through this recursive method, in addition to satisfying Berry's Eq. (S10), closely approximate the two actual eigenvalue-eigenvector pairs obtained by directly substituting $\hat{k}^\omega\left(\bar{k}_\rho\right)$ into Eq. (S9), provided the following additional condition identical to Brenier's[31] is met:

$$\mathrm{Im}\left[k^\omega\right] \neq k^\omega_{zI} = |\bar{k}^\omega_I| =: \underset{\sim}{k^\omega_I \ll k^\omega_R} := |\bar{k}^\omega_R| = \sqrt{k^2_\rho + k^2_{z\omega R}} \neq \mathrm{Re}\left[k^\omega\right], \tag{S12}$$

5 | *10, 11, 11, 11, 13.*

which can be easily fulfilled, because in most cases, material absorption is not strong enough to cause $k^\omega_I > k^\omega_R \cdot 10^{-3}$. On the contrary, even when materials exhibit strong absorption, there's no need to worry about theoretical inaccuracies because, in such cases, there is no transmitted light left to probe or investigate in the experiment.

One can prove that when Eq. (S12) is valid, the exact solution $k'^\omega(\hat{k}), \bar{d}'^\omega(\hat{k})$ of Eq. (S10), in combination with the iterative connection of Eq. (S11), which

results in $k'^{\omega}(\hat{k}(\bar{k}_{\rho}, k'^{\omega})), \bar{d}'^{\omega}(\hat{k}(\bar{k}_{\rho}, k'^{\omega}))$, numerically converges to the ground truth $k^{\omega}\left(\bar{k}_{\rho}\right), \bar{d}^{\omega}\left(\bar{k}_{\rho}\right)$ of Eq. (S9), by taking the limit of Eq. (S12), namely $k_{\mathrm{I}}^{\omega}=0$, which leads to Eq. (S10) fully equivalent to Eq. (S9) under the conditions of Eq. (S11), including both the equations themselves and their solutions, as demonstrated by[43].

A simple proof is as follows: Supposing $\bar{d}^{\omega} = \bar{d}'^{\omega} + \delta\bar{d}'^{\omega}$, substituting $\bar{d}'^{\omega} = \bar{d}^{\omega} - \delta\bar{d}'^{\omega}$ into both sides of Eq. (S10), and then substituting Eq. (S9) into the right side of Eq. (S10) under the assumption of Eq. (S11b), i.e. $n_{\omega}^2 = n_{\prime\omega}^2$, consequently, both sides cancel out $\bar{\bar{\eta}}^{\omega} \cdot \bar{d}^{\omega}$, yielding:

$$\left[\left(1-\hat{k}\hat{k}\right)\cdot\bar{\bar{\eta}}^{\omega}-\frac{1}{n_{\prime\omega}^{2}}\right]\cdot\delta\bar{d}'^{\omega}=\left(\hat{k}^{\omega}\hat{k}^{\omega}-\hat{k}\hat{k}\right)\cdot\bar{\bar{\eta}}^{\omega}\cdot\bar{d}^{\omega}, \tag{S13a}$$

$$\xrightarrow[\text{Eq. (S12)}]{\text{Eq. (S11a)}} \bar{0}, \tag{S13b}$$

in which $\hat{k}^{\omega} \to \hat{k} = \hat{k}_{\mathrm{R}}^{\omega}$ when both Eq. (S11a) and Eq. (S12) are satisfied, leading to $\delta\bar{d}'^{\omega} \parallel \bar{d}'^{\omega} \parallel \bar{d}^{\omega}$, which ultimately results in

$$\bar{g}'^{\omega} \parallel \bar{g}^{\omega} \tag{S14}$$

*3* | *13*, *24*, *25*.

through the constitutive relation $\bar{g}'^{\omega} = \bar{\bar{\eta}}^{\omega} \cdot \bar{d}'^{\omega}$ and $\bar{g}^{\omega} = \bar{\bar{\eta}}^{\omega} \cdot \bar{d}^{\omega}$.

Quoted @ *1* p. *23*.

## 2.2 Eigensystem pairs of non-uniform Fourier crystal optics

For the eigenvectors in non-uniform linear crystal Fourier optics(LFCO), one can obtain them without the need to set $\bar{d}^{\omega}\left(\bar{k}_{\rho}\right) \approx \bar{d}'^{\omega}(\hat{k}(\bar{k}_{\rho}, k'^{\omega}))$ — Once the eigenvalue is acquired through Eq. (S11b), it can be directly plugged into the nullspace of the two-rank system formed by three homogeneous linear equations[1, 7, 24, 44–46], namely Eq. (S5c) or Eq. (S6a) or Eq. (S9a), to produce the corresponding eigenvector. However, we refrained from employing such a method as Berry has presented a more elegant and paired resolution for the eigenvectors $\bar{d}'^{\omega}(\hat{k})$, with their physical significance being more explicitly stated.

For the eigenvalues in non-uniform LFCO, going a step further, we can map the connection between the complex wave vectors $k^{\omega}, k'^{\omega}$ in Eq. (S11) onto the interrelationships among the eigenvalue $k_{\mathrm{z}}^{\omega}$ in LFCO[1], Berry's refractive index $n'^{\omega}$, the effective refractive index $N^{\omega}$, polar angle $\theta^{\omega}$, and various related parameters, which will be eventually found consistent with the established conclusions for isotropic absorbing mediums[32]. Following this route, using $k_{\mathrm{z}}^{\omega} = k_{\mathrm{zR}}^{\omega} + \mathbb{i}k_{\mathrm{zI}}^{\omega}$ and $n'^{\omega} = n_{\mathrm{R}}'^{\omega} + \mathbb{i}n_{\mathrm{I}}'^{\omega}$, Eq. (S11b) can be further expressed as

$$k_{\rho}^{2} + k_{\mathrm{z}\omega}^{2} = k_{0\omega}^{2} n_{\prime\omega}^{2} \tag{S15a}$$

$$k_{\omega\mathrm{R}}^{2} - k_{\mathrm{z}\omega\mathrm{I}}^{2} + 2\mathbb{i}k_{\mathrm{zR}}^{\omega}k_{\mathrm{zI}}^{\omega} = k_{0\omega}^{2}\left(n_{\prime\omega\mathrm{R}}^{2} - n_{\prime\omega\mathrm{I}}^{2} + 2\mathbb{i}n_{\mathrm{R}}'^{\omega}n_{\mathrm{I}}'^{\omega}\right). \tag{S15b}$$

*1* | *12*.

Comparing the real and imaginary components of Eq. (S15b) above, one arrives at:

$$k_{\omega\mathrm{R}}^2 - k_{\omega\mathrm{I}}^2 = k_{0\omega}^2 \left(n_{\prime\omega\mathrm{R}}^2 - n_{\prime\omega\mathrm{I}}^2\right), \tag{S16a}$$
$$k_{\mathrm{zR}}^{\omega} k_{\mathrm{I}}^{\omega} = k_{0\omega}^2 n_{\mathrm{R}}^{\prime\omega} n_{\mathrm{I}}^{\prime\omega}. \tag{S16b}$$

If one defines

$$\begin{aligned}
\bar{k}^{\omega} &:= \bar{k}_{\mathrm{R}}^{\omega} + \mathbb{i}\bar{k}_{\mathrm{I}}^{\omega} && \text{(S17a)}\\
&= \left(k_{\mathrm{x}},\ k_{\mathrm{y}},\ k_{\mathrm{zR}}^{\omega}\right)^{\mathsf{T}} + \mathbb{i}\left(0,\ 0,\ k_{\mathrm{zI}}^{\omega}\right)^{\mathsf{T}} && \text{(S17b)}\\
&= k_{\mathrm{R}}^{\omega}\hat{k}_{\mathrm{R}}^{\omega} + \mathbb{i}k_{\mathrm{I}}^{\omega}\hat{\mathrm{e}}_{\mathrm{z}} && \text{(S17c)}\\
&:= k_0^{\omega}\left(N^{\omega}\hat{k}_{\mathrm{R}}^{\omega} + \mathbb{i}K^{\omega}\hat{\mathrm{e}}_{\mathrm{z}}\right), && \text{(S17d)}
\end{aligned}$$

where the *effective/apparent refractive indices* $(N^{\omega}, K^{\omega}) := \left(k_{\mathrm{R}}^{\omega}, k_{\mathrm{I}}^{\omega}\right)/k_0^{\omega}$, and

$$\begin{aligned}
\hat{k}_{\mathrm{R}}^{\omega} &= \mathcal{N}\left[\bar{k}_{\mathrm{R}}^{\omega}\right] = \left(\hat{k}_{\mathrm{xR}}^{\omega},\ \hat{k}_{\mathrm{yR}}^{\omega},\ \hat{k}_{\mathrm{zR}}^{\omega}\right)^{\mathsf{T}} && \text{(S18a)}\\
&= \left(k_{\mathrm{x}},\ k_{\mathrm{y}},\ k_{\mathrm{zR}}^{\omega}\right)^{\mathsf{T}}/k_{\mathrm{R}}^{\omega} && \text{(S18b)}\\
&:= \left(\sin\theta^{\omega}\cos\phi,\ \sin\theta^{\omega}\sin\phi,\ \cos\theta^{\omega}\right)^{\mathsf{T}}, && \text{(S18c)}
\end{aligned}$$

is set equivalent to Berry's $\hat{k}$ in Eq. (S11a), then Eq. (S16) becomes

$$N_{\omega}^2 - K_{\omega}^2 = n_{\prime\omega\mathrm{R}}^2 - n_{\prime\omega\mathrm{I}}^2, \tag{S19a}$$
$$N^{\omega}K^{\omega} = n_{\mathrm{R}}^{\prime\omega} n_{\mathrm{I}}^{\prime\omega}/\cos\theta^{\omega}, \tag{S19b}$$

which is a bi-quadratic equation of $N^{\omega}$, and the corresponding solution is

$$N^{\omega} = \sqrt{\frac{1}{2}\left[n_{\prime\omega\mathrm{R}}^2 - n_{\prime\omega\mathrm{I}}^2 + \sqrt{\left(n_{\prime\omega\mathrm{R}}^2 - n_{\prime\omega\mathrm{I}}^2\right)^2 + 4\left(n_{\mathrm{R}}^{\prime\omega} n_{\mathrm{I}}^{\prime\omega}/\cos\theta^{\omega}\right)^2}\,\right]}, \tag{S20a}$$
$$K^{\omega} = \frac{n_{\mathrm{R}}^{\prime\omega} n_{\mathrm{I}}^{\prime\omega}}{N^{\omega}\cos\theta^{\omega}}, \tag{S20b}$$

whose expression is in perfect alignment with that of isotropic absorbing materials[32], including the inhomogeneity angle $\theta^{\omega} = \arccos(\hat{k}_{\mathrm{R}}^{\omega}\cdot\hat{k}_{\mathrm{I}}^{\omega}) = \arccos(\hat{k}_{\mathrm{R}}^{\omega}\cdot\hat{\mathrm{e}}_{\mathrm{z}})$, which also functions as the polar angle of $\hat{k}_{\mathrm{R}}^{\omega}$ in the $\mathcal{Z}$ frame in this context. The only alteration is replacing the isotropic complex refractive index $n$ with Berry's anisotropic complex refractive index $n^{\prime\omega}$.

Hence, the complex eigenvalue $k_{\mathrm{z}}^{\omega}$ in non-uniform LFCO[1] can be written in the form of either Eq. (S8d) or

$$\begin{aligned}
k_{\mathrm{z}}^{\omega} &= k_{\mathrm{zR}}^{\omega} + \mathbb{i}k_{\mathrm{zI}}^{\omega} && \text{(S21a)}\\
&= k_{\mathrm{R}}^{\omega}\cos\theta^{\omega} + \mathbb{i}k_{\mathrm{I}}^{\omega} && \text{(S21b)}
\end{aligned}$$

*1* | *24.*

$$= k_0^\omega \left(N^\omega \cos\theta^\omega + \mathbb{i}K^\omega\right) \tag{S21c}$$
1 | 24.

$$= k_0^\omega \left(\sqrt{N_\omega^2 - NA_{0\omega}^2} + \mathbb{i}K^\omega\right) \tag{S21d}$$
1 | 13.

$$= \sqrt{k_{\omega\mathrm{R}}^2 - k_\rho^2} + \mathbb{i}k_\mathrm{I}^\omega. \tag{S21e}$$
3 | 13, 24, 24.

Between these two options, we tend to favor the former representation, as it offers a faster computational speed, because the loop chain along $\hat{k}_\mathrm{R}^\omega \to k^\omega \to k_\mathrm{z}^\omega \hookrightarrow k_{\mathrm{zR}}^\omega \to \bar{k}_\mathrm{R}^\omega \to \hat{k}_\mathrm{R}^\omega$ of Eq. (S11) is shorter than the one involving the effective refractive indices: $\hat{k}_\mathrm{R}^\omega \to k'^\omega \to n'^\omega \to N^\omega, K^\omega \to k_\mathrm{z}^\omega \hookrightarrow k_{\mathrm{zR}}^\omega \to \bar{k}_\mathrm{R}^\omega \to \hat{k}_\mathrm{R}^\omega$ (where $\hookrightarrow$ behaves much like a standard arrow, with the added function of serving as a separator). Nevertheless, we stress the importance of the latter pathway as it establishes a connection between the refractive index $n'^\omega$ along the real wave vectors $\bar{k}'^\omega = k'^\omega \hat{k} \in \mathbb{C}_\mathrm{r} \times \mathbb{R}_\ominus^2$ of Berry's uniform plane waves and the apparent refractive indices $N^\omega, K^\omega$ along the real and imaginary parts $\bar{k}_\mathrm{R}^\omega, \bar{k}_\mathrm{I}^\omega$ of the complex wave vectors $\bar{k}^\omega = \bar{k}_\mathrm{R}^\omega + \mathbb{i}\bar{k}_\mathrm{I}^\omega \in \mathbb{R}_\perp^2 + \mathbb{C}_\mathrm{Z}$ of non-uniform plane waves.

Keep in mind that, when dealing with Eq. (S20), always opt for the square root branch with a positive real part for both $N^\omega$ and $k_\mathrm{R}^\omega = k_0^\omega N^\omega$. This choice ensures its correspondence to $N^\omega, k_\mathrm{R}^\omega$ along the $\hat{k}_\mathrm{R}^\omega$ direction and simultaneously allows for $\theta^\omega > \pi/2$, where $k_{\mathrm{zR}}^\omega = k_\mathrm{R}^\omega \cos\theta^\omega < 0$, corresponding to the square root branch with a negative real part for Eqs. (S21d) and (S21e).

# 3 Supplementary Note 3

## 3.1 Transformations for vectors between $\mathcal{Z}, \mathcal{C}$ frames

In order to derive the eigenvalue-eigenvector pairs $k^\omega\left(\bar{k}_\rho\right), \bar{d}^\omega\left(\bar{k}_\rho\right) \approx k'^\omega(\hat{k}(\bar{k}_\rho, k'^\omega)), \bar{d}'^\omega(\hat{k}(\bar{k}_\rho, k'^\omega))$ of non-uniform LFCO within a confined slab material, it is crucial to have prior knowledge of the $\hat{k} - k'^\omega(\hat{k}), \bar{d}'^\omega(\hat{k})$ relationship of uniform plane waves in an unbounded medium. However, Berry did not directly provide solutions $k'^\omega(\hat{k}), \bar{d}'^\omega(\hat{k})$ for Eq. (S10) in the laboratory coordinate system (the $\mathcal{Z}$ frame); instead, the solutions $k'^\omega(\underline{\hat{k}}), \underline{\bar{d}}'^\omega(\underline{\hat{k}})$ for

$$\left(1 - \underline{\hat{k}}\underline{\hat{k}}\right) \cdot \underline{\bar{\bar{\eta}}}^\omega \cdot \underline{\bar{d}}'^\omega = \frac{1}{n_{\prime\omega}^2} \underline{\bar{d}}'^\omega, \tag{S22a}$$

$$\underline{\hat{k}} \cdot \underline{\bar{d}}'^\omega = 0, \tag{S22b}$$

were provided in the principal dielectric axis system (the $\mathcal{C}$ frame), whose axes $\underline{\hat{e}}_\mathrm{x}, \underline{\hat{e}}_\mathrm{y}, \underline{\hat{e}}_\mathrm{z}$ are along the principal axes of $\mathrm{Re}\,[\bar{\bar{\eta}}^\omega + \bar{\bar{\eta}}_\omega^\intercal]$. The only distinction between Eq. (S10) and Eq. (S22) is that in Eq. (S22), all vectors and tensors are marked with a short underscore _, signifying that they are measured in the $\mathcal{C}$ frame (except for $\underline{\hat{e}}_\mathrm{x}, \underline{\hat{e}}_\mathrm{y}, \underline{\hat{e}}_\mathrm{z}$ whose components are read in the $\mathcal{Z}$ frame); whereas in Eqs. (S1) to (S21), vectors and tensors are quantified in the $\mathcal{Z}$ frame for lacking an underscore _.

Seeking the yet-to-be-obtained eigenvalue-eigenvector pairs $k'^{\omega}(\hat{k}), \bar{d}'^{\omega}(\hat{k})$ of Eq. (S10) while possessing the available ones $k'^{\omega}(\underline{\hat{k}}), \underline{\bar{d}}'^{\omega}(\underline{\hat{k}})$ of Eq. (S22)[13] implies that additional efforts are required for coordinate transformations, such as $\underline{\hat{k}} \to \hat{k}$, $\underline{\bar{d}}'^{\omega} \to \bar{d}'^{\omega}$.

Assuming that the $\mathcal{C}$ frame coincides with the $\mathcal{Z}$ frame before any rotation and has the flexibility for arbitrary 3D rotations around the origin, denoted as

$$\overline{\underline{\hat{\mathrm{e}}}_{\curlywedge}} := \begin{pmatrix} \underline{\hat{\mathrm{e}}}_{\mathrm{x}} \\ \underline{\hat{\mathrm{e}}}_{\mathrm{y}} \\ \underline{\hat{\mathrm{e}}}_{\mathrm{z}} \end{pmatrix} := \underline{\bar{\bar{R}}}_{\curlywedge} \cdot \begin{pmatrix} \hat{\mathrm{e}}_{\mathrm{x}} \\ \hat{\mathrm{e}}_{\mathrm{y}} \\ \hat{\mathrm{e}}_{\mathrm{z}} \end{pmatrix} =: \underline{\bar{\bar{R}}}_{\curlywedge} \cdot \overline{\hat{\mathrm{e}}_{\curlywedge}} = \underline{\bar{\bar{R}}}_{\curlywedge}, \tag{S23}$$

where all quantities are measured in the rectangular ($\curlywedge$) coordinate $\mathcal{Z}$ frame, and the determination of $\overline{\underline{\hat{\mathrm{e}}}_{\curlywedge}} = \underline{\bar{\bar{R}}}_{\curlywedge}$ depends on the orientation of the non-orthogonal unit lattice vectors $\hat{a}, \hat{b}, \hat{c}$ (which establish the *crystallo-graphic coordinate system* (CCS) and commonly deviate from the three orthogonal basis vectors $\underline{\hat{\mathrm{e}}}_{\mathrm{x}}, \underline{\hat{\mathrm{e}}}_{\mathrm{y}}, \underline{\hat{\mathrm{e}}}_{\mathrm{z}}$ of the $\mathcal{C}$ frame[9, 41, 46]) and the specifics of crystal cuts (which determine $\hat{\mathrm{e}}_{\mathrm{z}}$ of the $\mathcal{Z}$ frame).

Here, $\overline{\hat{\mathrm{e}}_{\curlywedge}} = \left(\hat{\mathrm{e}}_{\mathrm{x}},\ \hat{\mathrm{e}}_{\mathrm{y}},\ \hat{\mathrm{e}}_{\mathrm{z}}\right)^{\mathsf{T}}$, which is also denoted as $\overline{\mathbf{e}_{\curlywedge}} = \left(\mathbf{e}_{\mathrm{x}},\ \mathbf{e}_{\mathrm{y}},\ \mathbf{e}_{\mathrm{z}}\right)^{\mathsf{T}}$, holding an extra continuous overline $^{-}$ across the entire symbol, is a “double vector”, with each of its components being a column vector.

The real rotation matrix $\underline{\bar{\bar{R}}}_{\curlywedge}$ converting both the real basis vectors $\underline{\bar{\bar{R}}}_{\curlywedge}$ for $\overline{\mathbf{e}_{\curlywedge}} \to \overline{\underline{\mathbf{e}}_{\curlywedge}}$ and its complex basis coefficients $\bar{v}_{\curlywedge} \to \underline{\bar{v}}_{\curlywedge}$ from the $\mathcal{Z}$ frame to the $\mathcal{C}$ frame[47]

$$\underline{\bar{v}}_{\curlywedge} = \begin{pmatrix} \underline{v}_{\mathrm{x}} \\ \underline{v}_{\mathrm{y}} \\ \underline{v}_{\mathrm{z}} \end{pmatrix} = \underline{\bar{\bar{R}}}_{\curlywedge} \cdot \begin{pmatrix} v_{\mathrm{x}} \\ v_{\mathrm{y}} \\ v_{\mathrm{z}} \end{pmatrix} = \underline{\bar{\bar{R}}}_{\curlywedge} \cdot \bar{v}_{\curlywedge}, \tag{S24}$$

under the rule of physical vectors being identical ones $\boldsymbol{v} = \underline{\boldsymbol{v}}$ regardless of measurement techniques

$$\bar{v}_{\curlywedge}^{\mathsf{T}} \cdot \overline{\mathbf{e}_{\curlywedge}} = \boldsymbol{v}_{\curlywedge} = \underline{\boldsymbol{v}}_{\curlywedge} = \underline{\bar{v}}_{\curlywedge}^{\mathsf{T}} \cdot \overline{\underline{\mathbf{e}}_{\curlywedge}}, \tag{S25}$$

can be realized in multiple forms, such as the Euler Angles method, the Axis-Angle approach and the Quaternion representation. Nevertheless, none of the methods mentioned above were employed. Rather, a rotation matrix

$$\underline{\bar{\bar{R}}}_{\curlywedge} = \underline{\bar{\bar{\mathcal{T}}}}_{\curlywedge} \cdot \underline{\bar{\bar{\mathcal{R}}}}_{\ominus} \cdot \bar{\bar{\mathcal{T}}}_{\ominus} \tag{S26}$$ *2* | *14, 16.*

was crafted by drawing insights from spherical trigonometry, providing a greater inclination toward spherical coordinates ($\ominus$) while maintaining compatibility with traditional Euler Angles methods.

The two operators/functions $\bar{\bar{\mathcal{T}}}_{\ominus}, \underline{\bar{\bar{\mathcal{T}}}}_{\curlywedge}$ in Eq. (S26) establishes the mathematical bridge for direction representation (of any real physical vector $\boldsymbol{v}$) between spherical ($\ominus$) and rectangular ($\curlywedge$) coordinate systems, provided that these two systems ($\ominus, \curlywedge$)

both belong to the same ($\mathcal{Z}$ or $\mathcal{C}$) frame:

$$\begin{pmatrix}\theta_{\boldsymbol{v}}\\ \phi_{\boldsymbol{v}}\end{pmatrix} =: \bar{\ominus}_{\boldsymbol{v}} := \bar{\bar{\mathcal{T}}}_{\ominus} \cdot \hat{v}_{\curlywedge} = \bar{\bar{\mathcal{T}}}_{\ominus} \cdot \begin{pmatrix}\hat{v}_{\mathrm{x}}\\ \hat{v}_{\mathrm{y}}\\ \hat{v}_{\mathrm{z}}\end{pmatrix} = \begin{pmatrix}\arccos \hat{v}_{\mathrm{z}}\\ \operatorname{arctan2}\left[\hat{v}_{\mathrm{y}}, \hat{v}_{\mathrm{x}}\right]\end{pmatrix} \tag{S27a}$$

*3* | *16*, *24*, *24*.

$$\begin{pmatrix}\hat{v}_{\mathrm{x}}\\ \hat{v}_{\mathrm{y}}\\ \hat{v}_{\mathrm{z}}\end{pmatrix} =: \hat{v}_{\curlywedge} := \bar{\bar{\mathcal{T}}}_{\curlywedge} \cdot \bar{\ominus}_{\boldsymbol{v}} = \bar{\bar{\mathcal{T}}}_{\curlywedge} \cdot \begin{pmatrix}\theta_{\boldsymbol{v}}\\ \phi_{\boldsymbol{v}}\end{pmatrix} = \begin{pmatrix}\sin\theta_{\boldsymbol{v}}\cos\phi_{\boldsymbol{v}}\\ \sin\theta_{\boldsymbol{v}}\sin\phi_{\boldsymbol{v}}\\ \cos\theta_{\boldsymbol{v}}\end{pmatrix}, \tag{S27b}$$

*2* | *16*, *16*.

where the four-quadrant arctangent $\operatorname{arctan2}[y, x]$ are adopted to preserve complete information of azimuthal angle $\phi$.

Being the central component of the rotation matrix, the operator $\bar{\bar{\underline{\mathcal{R}}}}_{\ominus}$ fully leverages the relevant principles of spherical trigonometry and facilitates a mathematical transition from the polar & azimuth angle $\theta_{\boldsymbol{v}}, \phi_{\boldsymbol{v}}$ measured in the $\mathcal{Z}$ frame to the ones $\underline{\theta}_{\boldsymbol{v}}, \underline{\phi}_{\boldsymbol{v}}$ measured in the $\mathcal{C}$ frame for the same real physical vector $\boldsymbol{v}$ ('s direction $\bar{\ominus}_{\boldsymbol{v}} \to \underline{\bar{\ominus}}_{\boldsymbol{v}}$):

$$\begin{aligned}\underline{\bar{\ominus}}_{\boldsymbol{v}} := \begin{pmatrix}\underline{\theta}_{\boldsymbol{v}}\\ \underline{\phi}_{\boldsymbol{v}}\end{pmatrix} := \bar{\bar{\underline{\mathcal{R}}}}_{\ominus} \cdot \begin{pmatrix}\theta_{\boldsymbol{v}}\\ \phi_{\boldsymbol{v}}\end{pmatrix} = \bar{\bar{\underline{\mathcal{R}}}}_{\ominus} \cdot \bar{\ominus}_{\boldsymbol{v}} \qquad \text{(S28a)}\\ = \begin{pmatrix}\arccos\left[\cos\theta_{\mathcal{C}}\cos\theta_{\boldsymbol{v}} + \sin\theta_{\mathcal{C}}\sin\theta_{\boldsymbol{v}}\cos\left(\phi_{\boldsymbol{v}} - \phi_{\mathcal{C}}\right)\right]\\ \operatorname{arctan2}\left[\sin\left(\phi_{\boldsymbol{v}} - \phi_{\mathcal{C}}\right), \cos\theta_{\mathcal{C}}\cos\left(\phi_{\boldsymbol{v}} - \phi_{\mathcal{C}}\right) - \sin\theta_{\mathcal{C}}\cot\theta_{\boldsymbol{v}}\right] - \underline{\phi}_{\mathcal{C}}\end{pmatrix}. \qquad \text{(S28b)}\end{aligned}$$

$\bar{\bar{\underline{\mathcal{R}}}}_{\ominus}$ requires 5 input parameters $\theta_{\boldsymbol{v}}, \phi_{\boldsymbol{v}}; \theta_{\mathcal{C}}, \phi_{\mathcal{C}}, \underline{\phi}_{\mathcal{C}}$ and generates 2 output parameters $\underline{\theta}_{\boldsymbol{v}}, \underline{\phi}_{\boldsymbol{v}}$. Among the 5 input parameters, 3 of them $\theta_{\mathcal{C}}, \phi_{\mathcal{C}}, \underline{\phi}_{\mathcal{C}}$ are exclusively tied to the crystal orientation (= the $\mathcal{C}$ frame orientation), that is, the orientation (relative pose) of the $\mathcal{C}$ frame with respect to the $\mathcal{Z}$ frame. Their numerical values are determined (unless encountering gimbal lock issues) once the slab material is affixed in the experimental setup and do not depend on the readings of vectors $\boldsymbol{v}$ undergoing coordinate transformation. As a result, the operator $\bar{\bar{\underline{\mathcal{R}}}}_{\ominus}$ can be viewed as a $2 \times 2$ function with both dual inputs $\theta_{\boldsymbol{v}}, \phi_{\boldsymbol{v}}$ and dual outputs $\underline{\theta}_{\boldsymbol{v}}, \underline{\phi}_{\boldsymbol{v}}$ expressed in spherical coordinates ($\ominus$).

It is specified that when $\theta_{\mathcal{C}}, \phi_{\mathcal{C}}, \underline{\phi}_{\mathcal{C}} = 0, 0, 0$, the $\mathcal{C}$ frame coincides with the $\mathcal{Z}$ frame. Then, the $\mathcal{C}$ frame is first rotated around the y axis of the $\mathcal{Z}$ frame, along the $\mathcal{Z}$ frame's z $\to$ x direction, by an polar angle of $\theta_{\mathcal{C}}$ relative to the $\mathcal{Z}$ frame's z axis. Subsequently, the $\mathcal{C}$ frame is rotated around the z axis of the $\mathcal{Z}$ frame, along the $\mathcal{Z}$ frame's x $\to$ y direction, by an azimuth angle of $\phi_{\mathcal{C}}$. Finally, the $\mathcal{C}$ frame is rotated around its own $\underline{\mathrm{z}}$ axis, along the $\mathcal{C}$ frame's $\underline{\mathrm{x}} \to \underline{\mathrm{y}}$ direction, by a self-rotation angle of $\underline{\phi}_{\mathcal{C}}$.

The rotation order described here can be abbreviated as $\mathrm{Y}(\theta_{\mathcal{C}})\mathrm{Z}(\phi_{\mathcal{C}})\underline{\mathrm{Z}}(\underline{\phi}_{\mathcal{C}})$, which is equivalent to $\underline{\mathrm{Y}}(\underline{\theta}_{\mathcal{C}})\mathrm{Z}(\phi_{\mathcal{C}})\underline{\mathrm{Z}}(\underline{\phi}_{\mathcal{C}})$, $\mathrm{Z}(\phi_{\mathcal{C}})\underline{\mathrm{Y}}(\underline{\theta}_{\mathcal{C}})\underline{\mathrm{Z}}(\underline{\phi}_{\mathcal{C}})$, and $\underline{\mathrm{Z}}(\underline{\phi}'_{\mathcal{C}})\underline{\mathrm{Y}}(\underline{\theta}_{\mathcal{C}})\underline{\mathrm{Z}}(\underline{\phi}_{\mathcal{C}})$, when it comes to the corresponding $\bar{\bar{\underline{R}}}_{\curlywedge}$, on condition that $\underline{\theta}_{\mathcal{C}}, \underline{\phi}'_{\mathcal{C}} = \theta_{\mathcal{C}}, \phi_{\mathcal{C}}$. Notably, among these 4 sequences $\mathrm{YZ}\underline{\mathrm{Z}}, \underline{\mathrm{Y}}\mathrm{Z}\underline{\mathrm{Z}}, \mathrm{Z}\underline{\mathrm{YZ}}, \underline{\mathrm{ZYZ}}$, the last approach $\underline{\mathrm{ZYZ}}$ is one of the 24 Euler angle methods, specifically categorized under the Proper Euler angle method

involving three consecutive internal rotations (right multiplications) in the local (current/dynamic/intrinsic) coordinate system $\mathcal{C}$.

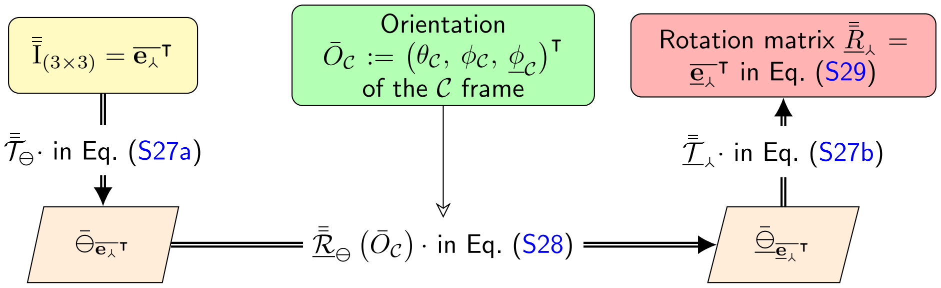


Quoted @ *6* pp. *23*, *25*, *28*, *29*, *29*, *29*.

**Fig. S1** Flowchart for Accessing $\underline{\bar{\bar{R}}}_{\curlywedge}\left(\bar{O}_{\mathcal{C}}\right)$ in Figs. S4, S5 and S6 as the output of Eq. (S29). For the meanings of styles of nodes & arrows, see Tables S1 and S2.

One can optimize the non-linear function Eq. (S26) by performing a single function stack call, applying $\underline{\bar{\bar{\mathcal{T}}}}_{\curlywedge} \cdot \underline{\bar{\bar{\mathcal{R}}}}_{\ominus} \cdot \bar{\bar{\mathcal{T}}}_{\ominus}$ to $\bar{\bar{\mathrm{I}}}_{(3\times3)} = \overline{\underline{\mathbf{e}}_{\curlywedge}}^{\mathsf{T}}$ to obtain the 2D real $3 \times 3$ array

$$\underline{\bar{\bar{R}}}_{\curlywedge} = \underline{\bar{\bar{R}}}_{\curlywedge} \cdot \bar{\bar{\mathrm{I}}}_{(3\times3)} = \underline{\bar{\bar{\mathcal{T}}}}_{\curlywedge} \cdot \underline{\bar{\bar{\mathcal{R}}}}_{\ominus} \cdot \bar{\bar{\mathcal{T}}}_{\ominus} \cdot \overline{\underline{\mathbf{e}}_{\curlywedge}}^{\mathsf{T}} \tag{S29}$$

*3* | *16*, *16*, *16*.

and store it in memory as a matrix with 9 constant coefficients, before transforming any other column vector $\bar{v}_{\curlywedge}$.

## 3.2 Transformations for vectors between $\curlywedge, \ominus$ coordinates

After acquiring the $3 \times 3$ rotation matrix $\underline{\bar{\bar{R}}}_{\curlywedge}$ from Eq. (S29), one also needs a $3 \times 2$ transformation matrix $\underline{\bar{\bar{\mathscr{T}}}}_{\curlywedge\ominus}$ that converts Berry's eigenvectors from the $\underline{\mathbf{e}}_{\theta}, \underline{\mathbf{e}}_{\phi}$ basis to the $\underline{\mathbf{e}}_{\mathrm{x}}, \underline{\mathbf{e}}_{\mathrm{y}}, \underline{\mathbf{e}}_{\mathrm{z}}$ basis and is addressed in the rectangular coordinate system ($\curlywedge$) by

$$\underline{\bar{\bar{\mathscr{T}}}}^{\curlywedge}_{\curlywedge\ominus} := \mathcal{T}_{\theta\phi}\left[\underline{\bar{\bar{\mathcal{T}}}}^{\curlywedge}_{\curlywedge\ominus}\right] = \left[\left(\bar{\mathrm{e}}_{\mathrm{z}} \times \underline{\hat{k}}_{\curlywedge}\right) \times \underline{\hat{k}}_{\curlywedge},\ \bar{\mathrm{e}}_{\mathrm{z}} \times \underline{\hat{k}}_{\curlywedge}\right] / \underline{\hat{k}}_{\rho}, \tag{S30}$$

*3* | *16*, *16*, *28*.

which shares the same characteristic with $\underline{\bar{\bar{\mathcal{T}}}}_{\curlywedge}$ from Eq. (S27b) in that it takes 2 parameters and provides 3 parameters.

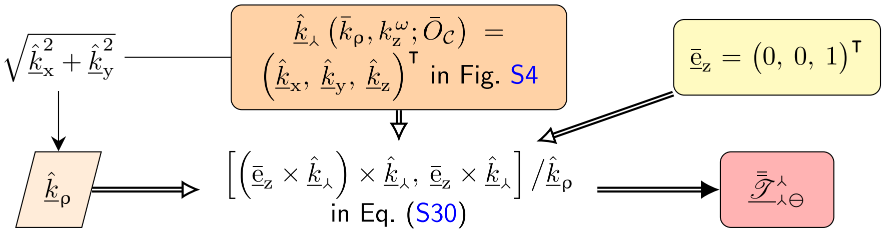


Quoted @ *6* pp. *23*, *25*, *28*, *29*, *29*, *29*.

**Fig. S2** Flowchart for Accessing $\underline{\bar{\bar{\mathscr{T}}}}^{\curlywedge}_{\curlywedge\ominus}\left(\underline{\hat{k}}_{\curlywedge}\right)$ in Fig. S6 as the output of Eq. (S30). For the meanings of styles of nodes & arrows, see Tables S1 and S2.

### 3.3 Conventions and relations for tensors $\bar{\bar{\eta}}^{\omega}, \bar{\bar{\varepsilon}}'^{\omega}_{\mathrm{r}}, \bar{\bar{\bar{\chi}}}^{(2)}_{\omega}$

Following Landau *et al.*[46] and Berry's[13] routine, we define $\bar{\bar{\epsilon}}^{\omega}, \bar{\bar{u}}^{\omega}$ as the symmetric part, namely $\frac{1}{2}\left[(\cdot)+(\cdot)^{\intercal}\right]$, of $\bar{\bar{\varepsilon}}'^{\omega}_{\mathrm{r}}, \bar{\bar{\eta}}^{\omega}$ (where $\bar{\bar{\epsilon}}^{\omega}$ contains symmetric $\frac{\mathbb{i}}{\varepsilon_0 \omega}\bar{\bar{\sigma}}^{\omega}$), describing the linear birefringence and linear dichroism of the material; and $\mathbb{i}\cdot\bar{\beta}^{\omega}\times, \mathbb{i}\cdot\bar{\alpha}^{\omega}\times$ as the antisymmetric part, namely $\frac{1}{2}\left[(\cdot)-(\cdot)^{\intercal}\right]$, of $\bar{\bar{\varepsilon}}'^{\omega}_{\mathrm{r}}, \bar{\bar{\eta}}^{\omega}$, describing the circular birefringence and circular dichroism which represent the simplest non-local response of the material[13], determined by the axial *gyration vector* $\bar{\beta}^{\omega}$, *optical activity vector* $\bar{\alpha}^{\omega}$[46].

Whether in the $\mathcal{Z}$ frame or the $\mathcal{C}$ frame, we adhere to:

$$\bar{\bar{\varepsilon}}'^{\omega}_{\mathrm{r}} := \bar{\bar{\epsilon}}^{\omega} + \mathbb{i}\cdot\bar{\beta}^{\omega}\times = \bar{\bar{\eta}}^{-1}_{\omega}, \tag{S31a}$$

$$\bar{\bar{\eta}}^{\omega} := \bar{\bar{u}}^{\omega} + \mathbb{i}\cdot\bar{\alpha}^{\omega}\times = \bar{\bar{\varepsilon}}'^{-1}_{\mathrm{r}\omega}, \tag{S31b}$$ 1 | 25.

in which $\bar{\bar{\epsilon}}^{\omega}, \bar{\beta}^{\omega}; \bar{\bar{u}}^{\omega}, \bar{\alpha}^{\omega}$ can be further specified as[46]

$$\bar{\bar{\epsilon}}^{\omega} = \frac{\bar{\bar{u}}^{-1}_{\omega}\det\left[\bar{\bar{u}}^{\omega}\right] - \bar{\alpha}^{\omega}\otimes\bar{\alpha}^{\omega}}{\det\left[\bar{\bar{\eta}}^{\omega}\right]}, \quad \bar{\beta}^{\omega} = -\frac{\bar{\bar{u}}^{\omega}}{\det\left[\bar{\bar{\eta}}^{\omega}\right]}\cdot\bar{\alpha}^{\omega}, \tag{S32a}$$

$$\bar{\bar{u}}^{\omega} = \frac{\bar{\bar{\epsilon}}^{-1}_{\omega}\det\left[\bar{\bar{\epsilon}}^{\omega}\right] - \bar{\beta}^{\omega}\otimes\bar{\beta}^{\omega}}{\det\left[\bar{\bar{\varepsilon}}'^{\omega}_{\mathrm{r}}\right]}, \quad \bar{\alpha}^{\omega} = -\frac{\bar{\bar{\epsilon}}^{\omega}}{\det\left[\bar{\bar{\varepsilon}}'^{\omega}_{\mathrm{r}}\right]}\cdot\bar{\beta}^{\omega}, \tag{S32b}$$

and can be reduced to a simpler form

$$\bar{\bar{\epsilon}}^{\omega} = \bar{\bar{u}}^{-1}_{\omega}, \quad \bar{\beta}^{\omega} = -\frac{\bar{\bar{u}}^{\omega}}{\det\left[\bar{\bar{u}}^{\omega}\right]}\cdot\bar{\alpha}^{\omega}, \tag{S33a}$$

$$\bar{\bar{u}}^{\omega} = \bar{\bar{\epsilon}}^{-1}_{\omega}, \quad \bar{\alpha}^{\omega} = -\frac{\bar{\bar{\epsilon}}^{\omega}}{\det\left[\bar{\bar{\epsilon}}^{\omega}\right]}\cdot\bar{\beta}^{\omega}, \tag{S33b}$$

only when either of the following two conditions holds:

$$|\bar{\bar{\epsilon}}^{\omega}_{\mathrm{R}}| \gg |\bar{\beta}^{\omega}_{\mathrm{R}}| \quad \text{and} \quad |\bar{\bar{\epsilon}}^{\omega}_{\mathrm{I}}| \gg |\bar{\beta}^{\omega}_{\mathrm{I}}|, \tag{S34a}$$

$$|\bar{\bar{u}}^{\omega}_{\mathrm{R}}| \gg |\bar{\alpha}^{\omega}_{\mathrm{R}}| \quad \text{and} \quad |\bar{\bar{u}}^{\omega}_{\mathrm{I}}| \gg |\bar{\alpha}^{\omega}_{\mathrm{I}}|, \tag{S34b}$$

which state that the average magnitudes of all tensor elements from the real/imaginary part of the antisymmetric part $\mathbb{i}\cdot\bar{\beta}^{\omega}\times$ ($\mathbb{i}\cdot\bar{\alpha}^{\omega}\times$), correspondingly, should be much smaller than that from the imaginary/real part (whose order is reversed) of the symmetric part $\bar{\bar{\epsilon}}^{\omega}$ ($\bar{\bar{u}}^{\omega}$) of $\bar{\bar{\varepsilon}}'^{\omega}_{\mathrm{r}}$ ($\bar{\bar{\eta}}^{\omega}$), where $\bar{\bar{\epsilon}}^{\omega}_{\mathrm{I}}$ includes the real symmetric conductivity tensor $\bar{\bar{\sigma}}^{\omega}$.

Regarding optical activity, in line with Berry's $\bar{g}^{\omega}$[13], Landau *et al.*'s $-\bar{G}^{\omega}$[46] and Bloembergen *et al.*'s $-\bar{\Gamma}^{\omega}$[48], we choose to first define the optical activity vector $\bar{\alpha}^{\omega}$, where $\bar{\alpha}^{\omega} := \bar{\bar{\gamma}}^{\omega}\cdot\hat{k}$ for natural optical activity depends linearly on the real wave vector direction $\hat{k}$, and $\bar{\alpha}^{\omega} := \bar{\bar{\gamma}}^{\omega}\cdot\bar{H}_{\mathrm{ex}}$ for Faraday rotation in magneto-optic materials[45, 46, 49] depends linearly on the external magnetic field $\bar{H}_{\mathrm{ex}}$, both proportional to the symmetric *optical activity tensor* $\bar{\bar{\gamma}}^{\omega}$.

One can also choose to define the gyration vector $\bar{\beta}^{\omega}$ as $\bar{\beta}^{\omega} := \bar{\bar{v}}^{\omega} \cdot \hat{k}$ or $\bar{\beta}^{\omega} := \bar{\bar{v}}^{\omega} \cdot \bar{H}$ with the corresponding symmetric *gyration tensor* $\bar{\bar{v}}^{\omega}$ rather than $\bar{\alpha}^{\omega}, \bar{\bar{\gamma}}^{\omega}$ as the first-hand description of optical activity, as taken by Landau *et al.*[46], Nelson[50, 51], Brenier[52], McLeod & Wagner[1], Belsky *et al.*[53] and Kuznetsov *et al.*[45, 49], rendering Eq. (S33) essential.

It's worth acknowledging that quantum electrodynamics[54] and recent studies[21, 22, 55, 56] both provide a non-phenomenological self-consistent derivation for the origin of natural optical activity, offering a more accurate nonlinear function of $\hat{k}$ for both $\bar{\beta}^{\omega} := n'^{\omega}(\hat{k})\bar{\bar{v}}^{\omega} \cdot \hat{k}$ and $\bar{\alpha}^{\omega} := n'^{\omega}(\hat{k})\bar{\bar{\gamma}}^{\omega} \cdot \hat{k}$, whose prediction deviates from $\bar{\beta}^{\omega} := \bar{\bar{v}}^{\omega} \cdot \hat{k}$ and $\bar{\alpha}^{\omega} := \bar{\bar{\gamma}}^{\omega} \cdot \hat{k}$ significantly only for propagation away from the optic axes of crystals possessing both large birefringence/anisotropy and strong optical activity.

Similar to Berry, in defining the Cartesian $\mathcal{C}$ frame (the dielectric principal axis system), we orient its three coordinate axes $\underline{\hat{e}}_{x}, \underline{\hat{e}}_{y}, \underline{\hat{e}}_{z}$ along the principal axes of $\bar{\bar{\epsilon}}_{R}^{\omega}$ in the Cartesian $\mathcal{Z}$ frame (where $\underline{\bar{\bar{\epsilon}}}_{R}^{\omega}$ in our $\mathcal{C}$ frame is diagonalized), which generally does not coincide[57] with the principal axes of $\bar{\bar{u}}_{R}^{\omega}$ adopted by Berry[13] (where $\underline{\bar{\bar{u}}}_{R}^{\omega}$ in Berry's $\mathcal{C}$ frame is diagonalized), unless either of the following two conditions is met:

$$|\underline{\bar{\bar{\epsilon}}}_{I}^{\omega}\text{ 's off-diagonal part}| \ll |\underline{\bar{\bar{\epsilon}}}_{R}^{\omega}| \quad \text{and} \quad |\underline{\bar{\beta}}_{R}^{\omega}| \ll |\underline{\bar{\bar{\epsilon}}}_{R}^{\omega}| \quad \text{and} \quad |\underline{\bar{\beta}}_{I}^{\omega}| \leq |\underline{\bar{\bar{\epsilon}}}_{R}^{\omega}|, \tag{S35a}$$

$$|\underline{\bar{\bar{u}}}_{I}^{\omega}\text{ 's off-diagonal part}| \ll |\underline{\bar{\bar{u}}}_{R}^{\omega}| \quad \text{and} \quad |\underline{\bar{\alpha}}_{R}^{\omega}| \ll |\underline{\bar{\bar{u}}}_{R}^{\omega}| \quad \text{and} \quad |\underline{\bar{\alpha}}_{I}^{\omega}| \leq |\underline{\bar{\bar{u}}}_{R}^{\omega}|, \tag{S35b}$$

this requirement can be readily satisfied[13, 31, 47, 48, 52], especially for the majority of natural dielectrics and common experimental settings. Thus, in most situations, Berry's $\mathcal{C}$ frame and our $\mathcal{C}$ frame largely overlap, rendering the re-diagonalization of $\underline{\bar{\bar{u}}}_{R}^{\omega}$ and the corresponding extra rotation of our $\mathcal{C}$ frame to Berry's $\mathcal{C}$ frame superfluous, and this permits the direct utilization of Berry's conclusions.

Our choice of this diagonal-$\underline{\bar{\bar{\epsilon}}}_{R}^{\omega}$ $\mathcal{C}$ frame is based on three key reasons. First, as mentioned above, to achieve the highest possible alignment with Berry's diagonal-$\underline{\bar{\bar{u}}}_{R}^{\omega}$ $\mathcal{C}$ frame, allowing for the direct inheritance of Berry's legacy[13]. Second, most literature provides Sellmeier equations for the three principal refractive indices $\underline{n}_{x}^{\omega}, \underline{n}_{y}^{\omega}, \underline{n}_{z}^{\omega} = \sqrt{\underline{\epsilon}_{Rxx}^{\omega}}, \sqrt{\underline{\epsilon}_{Ryy}^{\omega}}, \sqrt{\underline{\epsilon}_{Rzz}^{\omega}}$[31, 58–61] and high-order nonlinear coefficient tensors (e.g., $\underline{\bar{\bar{\bar{\chi}}}}_{\omega}^{(2)}$)[62, 63] in the diagonal-$\underline{\bar{\bar{\epsilon}}}_{R}^{\omega}$ $\mathcal{C}$ frame (i.e., the principal[9]/crystallo-optical[41] coordinate system (PCS)) as well, or in the crystal physics[9]/crystallo-physical[41]/piezoelectric[40, 47, 64] coordinate system (ZCS) that matches the PCS in 5/7 crystal systems[25, 30, 65]. Third, the calculation of effective nonlinear coefficients $\chi_{3\text{eff}}^{(2)\text{p}_{312}}$ from Eq. (6) in the main text is also commonly performed in this diagonal-$\underline{\bar{\bar{\epsilon}}}_{R}^{\omega}$ $\mathcal{C}$ frame[40, 41, 66, 67].

It is crucial to highlight that, the linear and nonlinear susceptibility tensors are originally specified in the ZCS[41, 47] among these four coordinate systems CCS $\to$ ZCS $\to$ PCS $\to$ LCS[9], where the latter three are right-handed orthogonal. Therefore, in order to minimize the number of non-zero elements in nonlinear coefficient tensors, the most appropriate model applicable to vector nonlinear crystal optics(NCO) should be built upon the ZCS, as opposed to the PCS we have currently selected, to avoid rotations on higher-order tensors and minimize the quantity of *for* loops.

However, in order to simplify the LCO section of the upcoming vector NCO while attempting not to increase the computational burden of its nonlinear optics(NO) section, we have chosen the PCS, referred to as the diagonal-$\underline{\bar{\bar{\epsilon}}}^{\omega}_{\mathrm{R}}$ $\mathcal{C}$ frame, for the primary intensive calculations in both the linear optics(LO) and NO parts. This allows the NO part of our model to perform computations with minimal additional cost for crystal systems with relatively higher symmetry, with the exception of the triclinic and monoclinic lattice systems, which exhibit the lowest symmetry where the corresponding ZCS usually do not coincide with the PCS, rendering rotations on higher-order tensors necessary[41], and the corresponding nonlinear coefficient tensors are more likely to contain a greater number of intrinsic non-zero elements even in the ZCS.

One must take into account that the PCS we utilize does not align with the principal axes of $\bar{\bar{\epsilon}}^{\omega}$[9, 33, 36] but those of $\bar{\bar{\epsilon}}^{\omega}_{\mathrm{R}}$, as complex symmetric matrices $\bar{\bar{\epsilon}}^{\omega}$ may not be diagonalizable via orthogonal similarity transformations, unlike real symmetric matrices $\bar{\bar{\epsilon}}^{\omega}_{\mathrm{R}}$. At most, they can only be (and sometimes still cannot be) diagonalized through unitary transformations by complex invertible matrices. As a result, the change-of-basis similarity transformation matrices for $\bar{\bar{\epsilon}}^{\omega}$ are usually complex, leading to all three coordinate axes of the $\mathcal{C}$ frame and their associated measurements being complex, with the degrees of freedom $(15-3+3)$ of the crystal's parameter space not reduced, as noted by Berry[13].

Moreover, we do not always adhere to Berry's prescribed order of the principal diagonal elements $\underline{u}^{\omega}_{\mathrm{Rxx}} > \underline{u}^{\omega}_{\mathrm{Ryy}} > \underline{u}^{\omega}_{\mathrm{Rzz}}$, namely $\underline{\epsilon}^{\omega}_{\mathrm{Rzz}} > \underline{\epsilon}^{\omega}_{\mathrm{Ryy}} > \underline{\epsilon}^{\omega}_{\mathrm{Rxx}}$, which expands as:

$$\begin{aligned}
\text{neg. uniaxial} &: \underline{n}^{\omega}_{\mathrm{z}} = \underline{n}^{\omega}_{\mathrm{y}} > \underline{n}^{\omega}_{\mathrm{x}} \;\; (\underline{n}^{\omega}_{\mathrm{o}} = \underline{n}^{\omega}_{\mathrm{z}})\,, && \text{(S36a)}\\
\text{pos. uniaxial} &: \underline{n}^{\omega}_{\mathrm{z}} > \underline{n}^{\omega}_{\mathrm{y}} = \underline{n}^{\omega}_{\mathrm{x}} \;\; (\underline{n}^{\omega}_{\mathrm{o}} = \underline{n}^{\omega}_{\mathrm{x}})\,, && \text{(S36b)}\\
\text{biaxial} &: \underline{n}^{\omega}_{\mathrm{z}} > \underline{n}^{\omega}_{\mathrm{y}} > \underline{n}^{\omega}_{\mathrm{x}}\,, && \text{(S36c)}\\
\text{neg.} &: \underline{n}^{\omega}_{\mathrm{z}} - \underline{n}^{\omega}_{\mathrm{y}} < \underline{n}^{\omega}_{\mathrm{y}} - \underline{n}^{\omega}_{\mathrm{x}}\,, && \text{(S36d)}\\
\text{pos.} &: \underline{n}^{\omega}_{\mathrm{z}} - \underline{n}^{\omega}_{\mathrm{y}} > \underline{n}^{\omega}_{\mathrm{y}} - \underline{n}^{\omega}_{\mathrm{x}}\,. && \text{(S36e)}
\end{aligned}$$

Instead, considering the convenience of numerical experiments and compatibility with mainstream crystal optics(CO), dielectric hyperbolic (meta)materials, and NCO, we have selected the following definition:

$$\begin{aligned}
\text{neg. uniaxial} &: |\underline{n}^{\omega}_{\mathrm{z}}| < \underline{n}^{\omega}_{\mathrm{y}} = \underline{n}^{\omega}_{\mathrm{x}} = \underline{n}^{\omega}_{\mathrm{o}}\,, && \text{(S37a)}\\
\text{pos. uniaxial} &: |\underline{n}^{\omega}_{\mathrm{z}}| > \underline{n}^{\omega}_{\mathrm{y}} = \underline{n}^{\omega}_{\mathrm{x}} = \underline{n}^{\omega}_{\mathrm{o}}\,, && \text{(S37b)}\\
\text{biaxial} &: |\underline{n}^{\omega}_{\mathrm{z}}| > \underline{n}^{\omega}_{\mathrm{y}} > \underline{n}^{\omega}_{\mathrm{x}}\,, && \text{(S37c)}\\
\text{neg. biaxial} &: |\underline{n}^{\omega}_{\mathrm{z}}| - \underline{n}^{\omega}_{\mathrm{y}} < \underline{n}^{\omega}_{\mathrm{y}} - \underline{n}^{\omega}_{\mathrm{x}}\,, && \text{(S37d)}\\
\text{pos. biaxial} &: |\underline{n}^{\omega}_{\mathrm{z}}| - \underline{n}^{\omega}_{\mathrm{y}} > \underline{n}^{\omega}_{\mathrm{y}} - \underline{n}^{\omega}_{\mathrm{x}}\,, && \text{(S37e)}
\end{aligned}$$

*1* | *20.*

where $|\cdot|$ denotes the modulus operation applied to complex numbers, and $\underline{n}^{\omega}_{\mathrm{o}}$ represents the refractive index of ordinary light. We have found that Berry's 2003 model[13] can be extended to accommodate materials with hyperbolic properties, allowing

$\underline{\epsilon}^{\omega}_{\mathrm{Rzz}} < 0$[14], that is, allowing $\underline{n}^{\omega}_{\mathrm{z}}$ to be purely imaginary, provided that $\underline{\epsilon}^{\omega}_{\mathrm{Rxx}}, \underline{\epsilon}^{\omega}_{\mathrm{Ryy}} > 0$ to ensure dielectric-type hyperbolic behavior.

Notably, for dielectric-type hyperbolic materials, the refractive index of the o-ray is always relatively smaller. As a result, in the case of negative uniaxial or biaxial materials, the o- and e-modes, as defined above in Eq. (S37a), should switch their respective references.

# 4 Supplementary Note 4

Quoted @ *2* pp. *23*, *23*.

## 4.1 Uniform plane waves in spherical $\mathcal{C}$ frame

In order to express his transverse matrix $\underline{\bar{\bar{m}}}'^{\omega}_{\theta\phi}$ gracefully, Berry introduced the "South-Pole Stereographic Projection" polar coordinate system. In this projection, the vector

$$\underline{\bar{R}} := \begin{pmatrix} \underline{X} \\ \underline{Y} \end{pmatrix} := \frac{\underline{\hat{k}}_{\rho}}{1+\underline{\hat{k}}_{\mathrm{z}}} := \frac{\left(\underline{\hat{k}}_{\mathrm{x}},\, \underline{\hat{k}}_{\mathrm{y}}\right)^{\mathsf{T}}}{1+\underline{\hat{k}}_{\mathrm{z}}} \tag{S38a}$$

*1* | *22*.

$$:= \sqrt{\frac{1-\underline{\hat{k}}_{\mathrm{z}}}{1+\underline{\hat{k}}_{\mathrm{z}}}} \begin{pmatrix} \cos\underline{\phi} \\ \sin\underline{\phi} \end{pmatrix} := \tan\frac{\underline{\theta}}{2} \begin{pmatrix} \cos\underline{\phi} \\ \sin\underline{\phi} \end{pmatrix} \tag{S38b}$$

*1* | *22*.

in the equatorial plane has its starting point at the center of the unit sphere, corresponding to the projection of the South Pole $-\underline{\mathbf{e}}_{\mathrm{z}}$ on the unit sphere. The endpoint of $\underline{\bar{R}}$ is determined by the intersection between the equatorial plane and the ray $\underline{\hat{k}}_{\curlywedge} + \underline{\mathbf{e}}_{\mathrm{z}}$ formed by the South Pole $-\underline{\mathbf{e}}_{\mathrm{z}} \to$ a certain point $\underline{\hat{k}}$ in the direction $\underline{\bar{\Theta}} = \left(\underline{\theta},\, \underline{\phi}\right)^{\mathsf{T}}$ on the unit sphere.

Alternatively, the real vector $\underline{\bar{R}}$ can be expressed using a complex scalar $\underline{Z}$, which is also composed of two independent real variables $\underline{X}, \underline{Y}$:

$$\underline{Z} = \underline{X} + \mathbb{i}\cdot\underline{Y}. \tag{S39}$$

*2* | *20*, *22*.

Using the representations of $\underline{\bar{R}}$ and $\underline{Z}$ obtained from Eqs. (S38) and (S39), the transverse matrix $\underline{\bar{\bar{m}}}'^{\omega}_{\theta\phi}$ becomes

$$\underline{\bar{\bar{m}}}'^{\omega}_{\theta\phi} = \frac{\underline{\bar{\bar{U}}}_{\phi\mathrm{L}} \cdot \begin{pmatrix} \underline{\mathcal{Q}}^{\omega} + \underline{\mathcal{G}}^{\omega} & \underline{\mathcal{P}}^{\omega}_{2} \\ \underline{\mathcal{P}}^{\omega}_{1} & \underline{\mathcal{Q}}^{\omega} - \underline{\mathcal{G}}^{\omega} \end{pmatrix} \cdot \underline{\bar{\bar{U}}}_{\mathrm{L}\phi}}{2\left(1+\underline{R}^{2}\right)^{2}}, \tag{S40}$$

*1* | *30*.

where the unitary matrix

$$\underline{\bar{\bar{U}}}_{\mathrm{L}\phi} = \frac{1}{\sqrt{2}} \begin{pmatrix} 1/\mathbb{e}^{\mathbb{i}\underline{\phi}} & -\mathbb{i}/\mathbb{e}^{\mathbb{i}\underline{\phi}} \\ 1\cdot\mathbb{e}^{\mathbb{i}\underline{\phi}} & \mathbb{i}\cdot\mathbb{e}^{\mathbb{i}\underline{\phi}} \end{pmatrix}, \tag{S41}$$

and four polynomials

$$
\begin{aligned}
\underline{\mathcal{Q}}^{\omega}\left(\underline{\bar{R}},\underline{\bar{\bar{u}}}^{\omega}\right) = {}& \left(1+\underline{R}^4\right)\left(\underline{u}^{\omega}_{\mathrm{xx}}+\underline{u}^{\omega}_{\mathrm{yy}}\right)+2\left(\underline{Y}^2-\underline{X}^2\right)\left(\underline{u}^{\omega}_{\mathrm{xx}}-\underline{u}^{\omega}_{\mathrm{yy}}\right) && \text{(S42a)} \\
& +4\underline{R}^2\underline{u}^{\omega}_{\mathrm{zz}}-8\underline{X}\underline{Y}\underline{u}^{\omega}_{\mathrm{xy}}-4\underline{X}\left(1-\underline{R}^2\right)\underline{u}^{\omega}_{\mathrm{xz}}-4\underline{Y}\left(1-\underline{R}^2\right)\underline{u}^{\omega}_{\mathrm{yz}}, \\
\underline{\mathcal{P}}^{\omega}_1\left(\underline{Z},\underline{\bar{\bar{u}}}^{\omega}\right) = {}& \underline{\mathcal{P}}^{\omega}_1\left(\underline{Z},\underline{\bar{\bar{u}}}^{\omega}_{\mathrm{R}}\right)+\mathbb{i}\cdot\underline{\mathcal{P}}^{\omega}_1\left(\underline{Z},\underline{\bar{\bar{u}}}^{\omega}_{\mathrm{I}}\right) && \text{(S42b)} \\
= {}& \left(1+\underline{Z}^4\right)\left(\underline{u}^{\omega}_{\mathrm{xx}}-\underline{u}^{\omega}_{\mathrm{yy}}\right)+2\underline{Z}^2\left(2\underline{u}^{\omega}_{\mathrm{zz}}-\underline{u}^{\omega}_{\mathrm{xx}}-\underline{u}^{\omega}_{\mathrm{yy}}\right) \\
& +2\mathbb{i}\cdot\left(1-\underline{Z}^4\right)\underline{u}^{\omega}_{\mathrm{xy}}-4\underline{Z}\left(1-\underline{Z}^2\right)\underline{u}^{\omega}_{\mathrm{xz}}-4\mathbb{i}\cdot\underline{Z}\left(1+\underline{Z}^2\right)\underline{u}^{\omega}_{\mathrm{yz}}, \\
\underline{\mathcal{P}}^{\omega}_2\left(\underline{Z},\underline{\bar{\bar{u}}}^{\omega}\right) = {}& \underline{\mathcal{P}}^{\omega *}_1\left(\underline{Z},\underline{\bar{\bar{u}}}^{\omega *}\right)=\underline{\mathcal{P}}^{\omega *}_1\left(\underline{Z},\underline{\bar{\bar{u}}}^{\omega}_{\mathrm{R}}\right)+\mathbb{i}\cdot\underline{\mathcal{P}}^{\omega *}_1\left(\underline{Z},\underline{\bar{\bar{u}}}^{\omega}_{\mathrm{I}}\right) && \text{(S42c)} \\
= {}& \left(1+\underline{Z}^{*4}\right)\left(\underline{u}^{\omega}_{\mathrm{xx}}-\underline{u}^{\omega}_{\mathrm{yy}}\right)+2\underline{Z}^{*2}\left(2\underline{u}^{\omega}_{\mathrm{zz}}-\underline{u}^{\omega}_{\mathrm{xx}}-\underline{u}^{\omega}_{\mathrm{yy}}\right) \\
& -2\mathbb{i}\cdot\left(1-\underline{Z}^{*4}\right)\underline{u}^{\omega}_{\mathrm{xy}}-4\underline{Z}^{*}\left(1-\underline{Z}^{*2}\right)\underline{u}^{\omega}_{\mathrm{xz}}+4\mathbb{i}\cdot\underline{Z}^{*}\left(1+\underline{Z}^{*2}\right)\underline{u}^{\omega}_{\mathrm{yz}}, \\
\underline{\mathcal{G}}^{\omega}\left(\underline{\bar{R}},\underline{\bar{\alpha}}^{\omega}\right) = {}& 2\left(1+\underline{R}^2\right)^2\underline{\bar{\alpha}}^{\omega}\cdot\underline{\hat{k}} && \text{(S42d)} \\
\xrightarrow{\underline{\bar{\alpha}}^{\omega}=\underline{\bar{\bar{\gamma}}}^{\omega}\cdot\underline{\hat{k}}} {}& 2\Big[4\underline{X}^2\underline{\gamma}^{\omega}_{\mathrm{xx}}+4\underline{Y}^2\underline{\gamma}^{\omega}_{\mathrm{yy}}+\left(1-\underline{R}^2\right)^2\underline{\gamma}^{\omega}_{\mathrm{zz}} \\
& +8\underline{X}\underline{Y}\underline{\gamma}^{\omega}_{\mathrm{xy}}+4\left(1-\underline{R}^2\right)\left(\underline{X}\underline{\gamma}^{\omega}_{\mathrm{xz}}+\underline{Y}\underline{\gamma}^{\omega}_{\mathrm{yz}}\right)\Big].
\end{aligned}
$$

(S42a) 1 | 22. (S42b) 1 | 22. (S42c) 1 | 22. (S42d) 1 | 22.

The eigenvalues of $\underline{\bar{\bar{m}}}'^{\omega}_{\theta\phi}$ then can be expressed using $\underline{\mathcal{Q}}^{\omega},\underline{\mathcal{P}}^{\omega}_1,\underline{\mathcal{P}}^{\omega}_2,\underline{\mathcal{G}}^{\omega}$ with $\underline{\bar{R}},\underline{Z},\underline{\bar{\bar{u}}}^{\omega},\underline{\bar{\alpha}}^{\omega}$:

$$
\left.\frac{1}{n'^2_{\omega}}\right|_{\pm}=\frac{\underline{\mathcal{Q}}^{\omega}\pm\underline{\Delta}^{\omega}}{2\left(1+\underline{R}^2\right)^2},\quad \underline{\Delta}^{\omega}:=\sqrt{\underline{\mathcal{P}}^{\omega}_1\underline{\mathcal{P}}^{\omega}_2+\underline{\mathcal{G}}^2_{\omega}}, \tag{S43}
$$

1 | 22.

where the two refractive indices along the direction of $\underline{\hat{k}}$ in the $\mathcal{C}$ frame (or $\hat{k}$ in the $\mathcal{Z}$ frame) are given by:

$$
n'^{\omega}_{\pm}=\frac{\sqrt{2}\left(1+\underline{R}^2\right)}{\sqrt{\underline{\mathcal{Q}}^{\omega}\mp\underline{\Delta}^{\omega}}}. \tag{S44}
$$

2 | 22, 22.

The process of obtaining a specific refractive index $n'^{\omega}_{+}$ or $n'^{\omega}_{-}$ involves square root operations twice on complex numbers, with the consistent choice of the branch where the real part is positive each time, consistent with Berry[13].

Using Eq. (S41), the two representations $\underline{\bar{d}}'^{\omega\pm}_{1\theta\phi},\underline{\bar{d}}'^{\omega\pm}_{2\theta\phi}$ of the two eigenvectors $\underline{\bar{d}}'^{\omega\pm}_{\theta\phi}$ of the transverse matrix $\underline{\bar{\bar{m}}}'^{\omega}_{\theta\phi}$ are derived to be:

$$
\begin{pmatrix}\underline{\bar{d}}'^{\omega\pm}_{1\theta\phi} & \underline{\bar{d}}'^{\omega\pm}_{2\theta\phi}\end{pmatrix}=\begin{pmatrix}1\cdot\mathbb{e}^{\mathbb{i}\underline{\phi}} & 1/\mathbb{e}^{\mathbb{i}\underline{\phi}}\\ \mathbb{i}\cdot\mathbb{e}^{\mathbb{i}\underline{\phi}} & -\mathbb{i}/\mathbb{e}^{\mathbb{i}\underline{\phi}}\end{pmatrix}\begin{pmatrix}\pm\underline{\Delta}^{\omega}+\underline{\mathcal{G}}^{\omega} & \underline{\mathcal{P}}^{\omega}_2\\ \underline{\mathcal{P}}^{\omega}_1 & \pm\underline{\Delta}^{\omega}-\underline{\mathcal{G}}^{\omega}\end{pmatrix}, \tag{S45}
$$

where normalization is temporarily excluded.

Moreover, owing to the property of linear combinations among eigenvectors belonging to the same eigenvalue still sharing that eigenvalue, the third and fourth

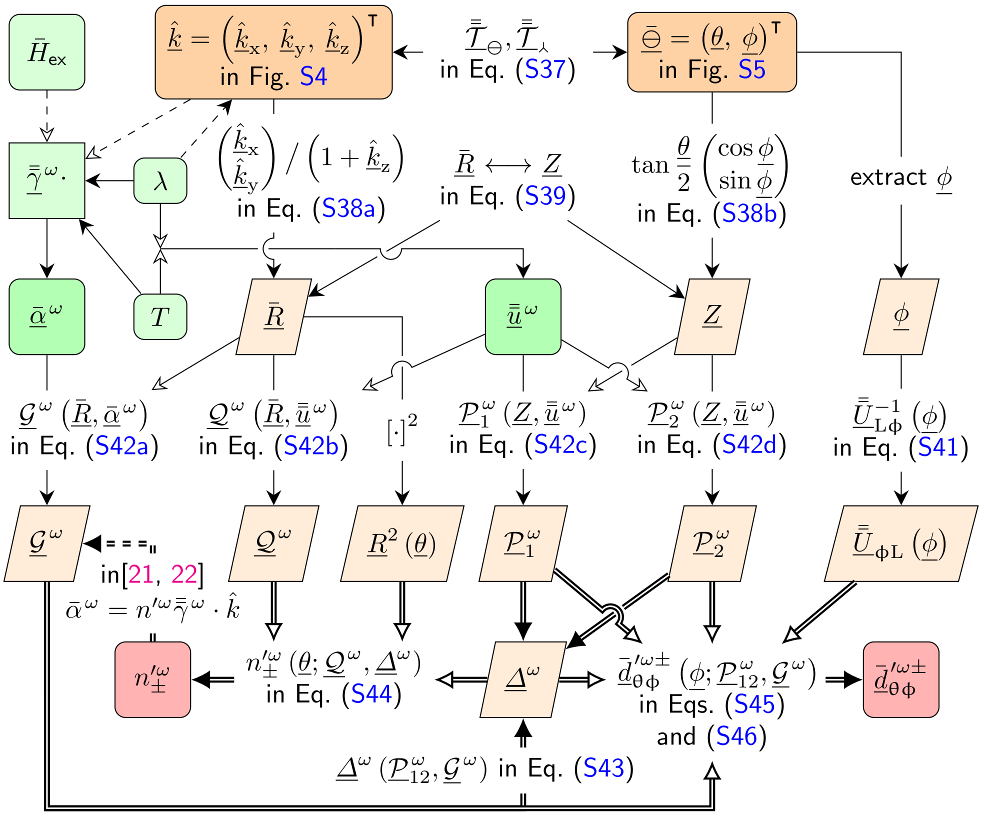


Quoted @ *13* pp. *22*, *23*, *23*, *23*, *24*, *24*, *24*, *25*, *25*, *28*, *29*, *29*, *29*.

**Fig. S3** Flowchart for Accessing $n'^{\omega}_{\pm}\left(\underline{\hat{k}} \text{ or } \underline{\bar{\ominus}}; \underline{\bar{u}}^{\omega}, \underline{\bar{\alpha}}^{\omega}\right)$ in Figs. S4 and S5 as the output of Eq. (S44), and $\underline{\bar{d}}'^{\omega\pm}_{\theta\phi}\left(\underline{\hat{k}} \text{ or } \underline{\bar{\ominus}}; \underline{\bar{u}}^{\omega}, \underline{\bar{\alpha}}^{\omega}\right)$ in Fig. S6 as the output of Eqs. (S45) and (S46). For the meanings of styles of nodes & arrows, see Tables S1 and S2.

representations $\underline{\bar{d}}'^{\omega\pm}_{3\theta\phi}, \underline{\bar{d}}'^{\omega\pm}_{4\theta\phi}$ of $\underline{\bar{d}}'^{\omega\pm}_{\theta\phi}$ can be established:

$$\left(\underline{\bar{d}}'^{\omega\pm}_{3\theta\phi} \;\; \underline{\bar{d}}'^{\omega\pm}_{4\theta\phi}\right) = \begin{pmatrix} 1\cdot \mathrm{e}^{\mathrm{i}\underline{\phi}} & 1/\mathrm{e}^{\mathrm{i}\underline{\phi}} \\ \mathrm{i}\cdot \mathrm{e}^{\mathrm{i}\underline{\phi}} & -\mathrm{i}/\mathrm{e}^{\mathrm{i}\underline{\phi}} \end{pmatrix} \begin{pmatrix} \pm\underline{\Delta}^{\omega} + \mathcal{G}^{\omega} & \mathcal{P}_2^{\omega} \\ \mathcal{P}_1^{\omega} & \pm\underline{\Delta}^{\omega} - \mathcal{G}^{\omega} \end{pmatrix} \begin{pmatrix} 1/\mathrm{e}^{\mathrm{i}\underline{\phi}} & -\mathrm{i}/\mathrm{e}^{\mathrm{i}\underline{\phi}} \\ 1\cdot \mathrm{e}^{\mathrm{i}\underline{\phi}} & \mathrm{i}\cdot \mathrm{e}^{\mathrm{i}\underline{\phi}} \end{pmatrix}. \tag{S46}$$

The four forms of $\underline{\bar{d}}'^{\omega\pm}_{\theta\phi} \in \underline{\mathbb{C}}^2_{\ominus}$ in Eqs. (S45) and (S46) are considered equivalent due to the parallelism $\underline{\bar{d}}'^{\omega\pm}_{1\theta\phi} \parallel \underline{\bar{d}}'^{\omega\pm}_{2\theta\phi} \parallel \underline{\bar{d}}'^{\omega\pm}_{3\theta\phi} \parallel \underline{\bar{d}}'^{\omega\pm}_{4\theta\phi}$.

The method to obtain eigensystem (eigenvalue-vector pairs) of uniform plane waves in spherical $\mathcal{C}$ frame $n'^{\omega}(\underline{\hat{k}}), \underline{\bar{d}}'^{\omega}_{\theta\phi}(\underline{\hat{k}}) \in \underline{\mathbb{C}}_{\mathrm{r}}\left(\underline{\mathbb{R}}^2_{\ominus}\right), \underline{\mathbb{C}}^2_{\ominus}\left(\underline{\mathbb{R}}^2_{\ominus}\right)$ has now been furnished by Fig. S3.

### 4.2 Non-uniform Fourier crystal optics in rectangular $\mathcal{Z}$ frame

Following the guiding principles of Eq. (S11), we now attempt to incorporate Berry's uniform eigenvalues and eigenvectors in spherical $\mathcal{C}$ frame $n'^{\omega}(\hat{\underline{k}}), \underline{\bar{d}}'^{\omega}_{\theta\phi}(\hat{\underline{k}}) \in \underline{\mathbb{C}}_{\mathrm{r}}\left(\mathbb{R}^2_{\ominus}\right), \underline{\mathbb{C}}^2_{\ominus}\left(\mathbb{R}^2_{\ominus}\right)$ from the previous Section 4.1 into eigenvalue-eigenvector pairs in Cartesian $\mathcal{Z}$ frame $k^{\omega}_{\mathrm{z}}\left(\bar{k}_{\rho}\right), \bar{d}^{\omega}_{\curlywedge}\left(\bar{k}_{\rho}\right) \in \mathbb{C}_{\mathrm{z}}\left(\mathbb{R}^2_{\rho}\right), \mathbb{C}^3_{\curlywedge}\left(\mathbb{R}^2_{\rho}\right)$ within the framework of non-uniform LFCO. Both the independent variables (inputs) $\hat{\underline{k}} \to \bar{k}_{\rho}$ and dependent variables (outputs) $n'^{\omega}, \underline{\bar{d}}'^{\omega}_{\theta\phi} \to k^{\omega}_{\mathrm{z}}, \bar{d}^{\omega}_{\curlywedge}$ of the eigenvalue-eigenvector pairs will undergo this transformation.

For eigenvalues, the detailed expansion from uniform complex wave vectors in unbounded media in spherical $\mathcal{C}$ frame $\bar{k}'^{\omega}(\hat{\underline{k}}) := k'^{\omega}(\hat{\underline{k}})\hat{\underline{k}} := k^{\omega}_0 n'^{\omega}(\hat{\underline{k}})\hat{\underline{k}} \in \underline{\mathbb{C}}_{\mathrm{r}}\left(\mathbb{R}^2_{\ominus}\right) \times \mathbb{R}^2_{\ominus}$[13], to non-uniform complex wave vectors $\bar{k}^{\omega}\left(\bar{k}_{\rho}\right) := \bar{k}_{\perp}\left(\bar{k}_{\rho}\right) + \bar{k}^{\omega}_{\mathrm{z}}\left(\bar{k}_{\rho}\right) \in \mathbb{R}^2_{\perp}\left(\mathbb{R}^2_{\rho}\right) + \mathbb{C}_{\mathrm{Z}}\left(\mathbb{R}^2_{\rho}\right)$[1] in confined media in rectangular $\mathcal{Z}$ frame, can be elaborated by extending the cyclic chain $\hat{k}^{\omega}_{\mathrm{R}} \to k^{\omega} \to k^{\omega}_{\mathrm{z}} \hookrightarrow k^{\omega}_{\mathrm{zR}} \to \bar{k}^{\omega}_{\mathrm{R}} \to \hat{k}^{\omega}_{\mathrm{R}}$ at the end of Section 2.1 and integrating the realization of Fig. S3 at the end of Section 4.1. The resulting algorithm flowchart is illustrated in Fig. S4.

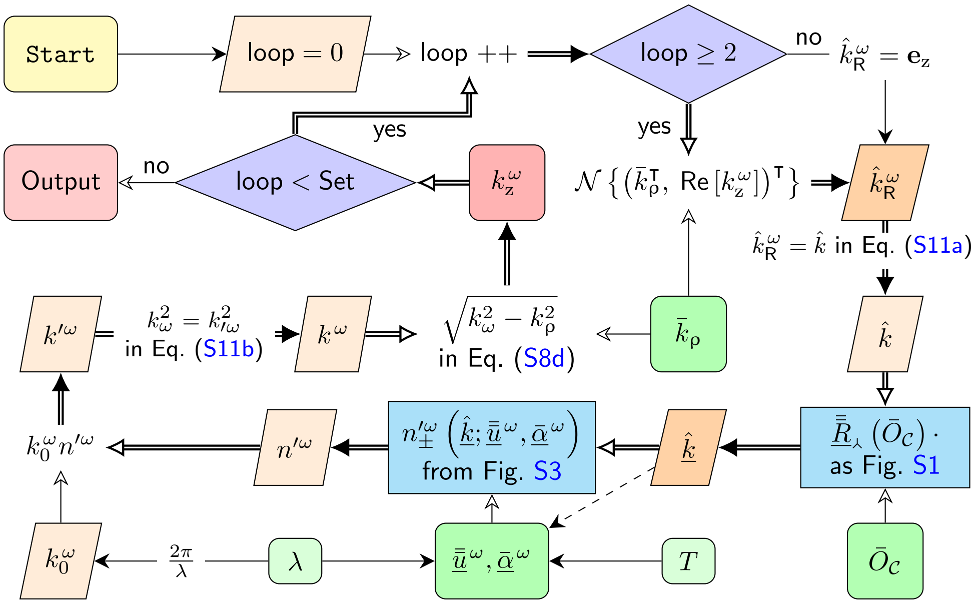


Quoted @ *17* pp. *16*, *16*, *22*, *22*, *23*, *23*, *24*, *24*, *25*, *25*, *27*, *28*, *28*, *28*, *29*, *29*, *29*.

**Fig. S4** Flowchart for Accessing $k^{\omega}_{\mathrm{z}}\left(\bar{k}_{\rho}; \bar{\bar{u}}^{\omega}, \bar{\alpha}^{\omega}; \bar{O}_{\mathcal{C}}\right)$ in Fig. S7 as the output of Eq. (S8d), together with $\hat{\underline{k}}^{\omega}_{\mathrm{R}} = \hat{\underline{k}}\left(\bar{k}_{\rho}, k^{\omega}_{\mathrm{z}}; \bar{O}_{\mathcal{C}}\right)$ in Figs. S2, S3, S6 and S7. For the meanings of styles of nodes & arrows, see Tables S1 and S2.

We temporarily do not emphasize the property that $n'^{\omega}_{\pm}$ has $\pm$ two modes, to make the flowchart easier to comprehend and reduce its complexity. Attention must be given to the fact that for each mode $+/-$ , a corresponding loop in Fig. S4 must

be executed separately, and the mode $+/-$ of $n'^{\omega}_{\pm}\left(\hat{\underline{k}};\bar{\underline{u}}^{\omega},\underline{\alpha}^{\omega}\right)$ from Fig. S3 should remain unchanged throughout its loop to acquire the corresponding correct $k^{\omega}_{z}\left(\bar{k}_{\rho}\right)$, which shares the same $\bar{k}_{\rho}$ grid with its counterpart mode.

To align the entire process in Fig. S4 more closely with spherical coordinate systems ($\ominus$) and simultaneously acquire the stored effective refractive indices $N^{\omega}$ and $K^{\omega}$ within the *effective/apparent wave vector* (much like $k^{\omega}_{z}$ from Eqs. (S21b) and (S21c))

$$\mathfrak{K}^{\omega} := k^{\omega}_{\mathrm{R}} + \mathbb{i}k^{\omega}_{\mathrm{I}} \tag{S47a}$$

$$= k^{\omega}_{0}\left(N^{\omega} + \mathbb{i}K^{\omega}\right), \tag{S47b}$$

Fig. S3 can be combined with different loop chains, such as $\bar{\ominus}^{\omega} \to n'^{\omega} \to N^{\omega} \hookrightarrow \theta^{\omega} \to \bar{\ominus}^{\omega}$, leading to another flowchart in Fig. S5, equivalent to Fig. S4.

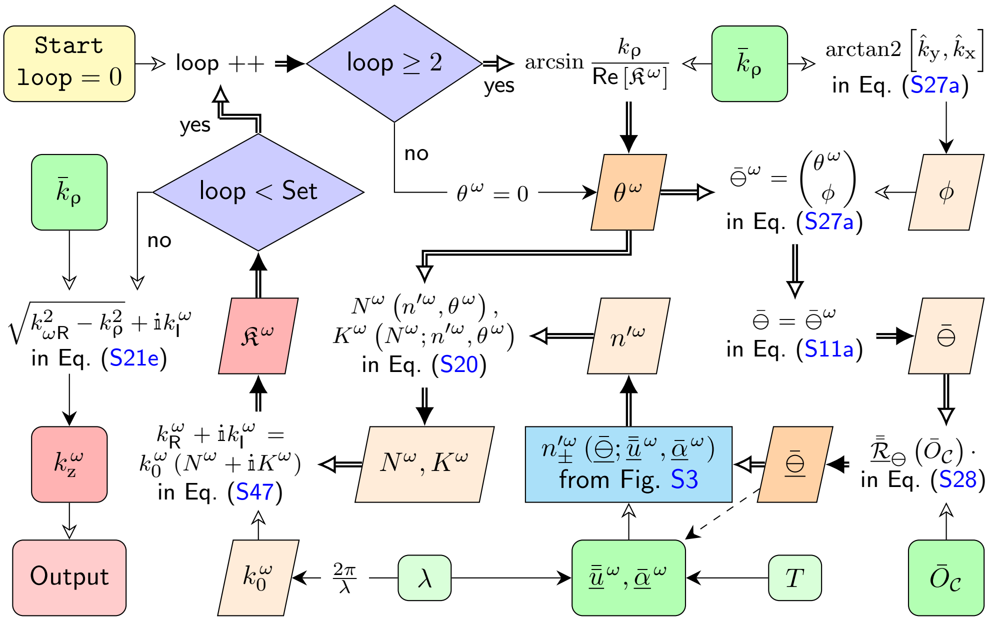


Quoted @ 9 pp. 16, 22, 22, 24, 27, 28, 29, 29, 29.

**Fig. S5** Flowchart for Accessing $k^{\omega}_{z}\left(\bar{k}_{\rho};\bar{\underline{u}}^{\omega},\underline{\alpha}^{\omega};\bar{O}_{\mathcal{C}}\right)$ in Fig. S7 as the output of Eq. (S21e), together with $\mathfrak{K}^{\omega}\left(\bar{k}_{\rho};\bar{\underline{u}}^{\omega},\underline{\alpha}^{\omega};\bar{O}_{\mathcal{C}}\right)$ for $N^{\omega}, K^{\omega}$ analysis as the output of Eq. (S47). For the meanings of styles of nodes & arrows, see Tables S1 and S2.

Concerning the eigenvectors of the electric field, we can streamline the entire derivation $\bar{\underline{d}}'^{\omega}_{\theta\phi} \to \bar{\underline{d}}'^{\omega}_{\curlywedge} \to \bar{d}^{\omega}_{\curlywedge} \to \bar{g}^{\omega}_{\curlywedge}$ or $\bar{\underline{d}}'^{\omega}_{\theta\phi} \to \bar{\underline{d}}^{\omega}_{\curlywedge} \to \bar{\underline{g}}^{\omega}_{\curlywedge} \to \bar{g}^{\omega}_{\curlywedge}$ (it's evident that certain operators are commutative) and represent it in a concise manner:

$$\bar{g}^{\omega\pm}_{\curlywedge} \xleftarrow[\text{in Eq. (S14)}]{\bar{g}^{\omega}\|\bar{g}'^{\omega}} \bar{\bar{R}}_{\curlywedge}\cdot\bar{\bar{\underline{\eta}}}^{\omega}_{\curlywedge}\cdot\bar{\bar{\underline{\mathscr{T}}}}^{\curlywedge}_{\curlywedge\ominus}\cdot\bar{\underline{d}}'^{\omega\pm}_{\theta\phi}, \tag{S48}$$ 3 | 25, 26, 30.

which can be further represented in the form of a flowchart in Fig. S6.

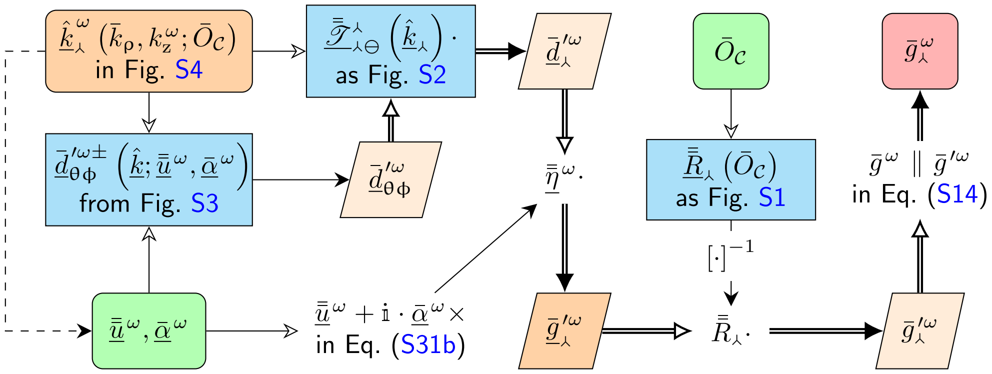


Quoted @ *14* pp. *16*, *16*, *22*, *23*, *25*, *25*, *25*, *25*, *27*, *28*, *28*, *29*, *29*, *29*.

**Fig. S6** Flowchart for Accessing $\bar{g}_{\curlywedge}^{\omega}\left(\bar{k}_{\rho}; \bar{\bar{\underline{u}}}^{\omega}, \underline{\bar{\alpha}}^{\omega}; \bar{O}_{\mathcal{C}}\right)$ in Fig. S7 as the output of Eq. (S48). For the meanings of styles of nodes & arrows, see Tables S1 and S2.

Again, the fact that $\bar{g}_{\curlywedge}^{\omega}$ has $\pm$ two modes has been temporarily excluded from the flowchart in Fig. S6 to minimize mental burden. Additionally, for each mode $+/-$ of $\hat{\underline{k}}_{\curlywedge}^{\omega}\left(\bar{k}_{\rho}, k_z^{\omega}; \bar{O}_{\mathcal{C}}\right)$ in Fig. S4 as one of the inputs of Fig. S6, one must choose the corresponding algorithm $\underline{\bar{d}}_{\theta\phi}^{\prime\omega\pm}\left(\hat{\underline{k}}; \bar{\bar{\underline{u}}}^{\omega}, \underline{\bar{\alpha}}^{\omega}\right)$ from Fig. S3 with the same mode, in order to attain the corresponding correct polarization state $\bar{g}_{\curlywedge}^{\omega}\left(\bar{k}_{\rho}\right)$ of the same mode. Furthermore, the polarization states $\underline{\bar{g}}_{\curlywedge}^{\omega} \parallel \underline{\bar{g}}_{\curlywedge}^{\prime\omega}$ under the rectangular $\mathcal{C}$ frame, serving as a cornerstone in the intermediate process of Fig. S6, will play a crucial role in subsequent vector NFCO.

Apart from the polarization states $\bar{g}_{\curlywedge}^{\omega\pm}$ of the Cartesian $\mathcal{Z}$-frame electric field within the crystal ($0 < z < L$), we present the pseudo-polarization states $\bar{g}_{\curlywedge}^{\omega\mathrm{i}}$ or $\bar{d}_{\curlywedge}^{\omega\mathrm{i}}$ inside a uniaxial crystal with strong linear dichroism along $\perp \mathbf{e}_{\mathrm{i}}$ direction acting as the linear polarizer/analyzer outside the crystal ($z < 0$ or $z > L$):

$$\bar{g}_{\curlywedge}^{\omega\mathrm{i}} := \bar{d}_{\curlywedge}^{\omega\mathrm{i}} := \left(\bar{k}_0^{\omega} \times \mathbf{e}_{\mathrm{i}}\right) \times \bar{k}_0^{\omega}, \qquad \mathrm{i} = \mathrm{x}, \mathrm{y}... = \leftharpoondown, \upharpoonleft, ..., \tag{S49}$$ *1* | *25.*

with $\bar{k}_0^{\omega} = \left(k_{\mathrm{x}},\ k_{\mathrm{y}},\ k_{0\mathrm{z}}^{\omega}\right)^{\intercal}$ where $k_{0\mathrm{z}}^{\omega} = \sqrt{k_{0\omega}^2 - k_{\rho}^2}$.

The pseudo-polarization state $\bar{g}_{\curlywedge}^{\omega\mathrm{i}}$ from Eq. (S49) of the analyzer only transmits light whose polarization state is parallel to $\bar{g}_{\curlywedge}^{\omega\mathrm{i}}$, and thus simplifies the incorporation of polarization crosstalk effects in non-paraxial cases during polarization analysis[68], while ensuring the relative authenticity (physicality) and accuracy of the simulation of this effect.

# 5 Supplementary Note 5

## 5.1 The transition matrix field constructed by the superimposed electric vector field's spatiotemporal spectrum

Up to Eq. (S48), we have established the eigensystem $k_{\pm}^{\omega}, \bar{g}_{\curlywedge}^{\omega\pm}$ of Eqs. (S6) and (S10), where both the independent and dependent variables are in the $\mathcal{Z}$ frame. This allows us to write the *general solution* $\bar{g}_{\curlywedge}^{\omega}$ to Eqs. (S6) and (S10) as a linear superposition of paired eigenvectors $\bar{g}_{\curlywedge}^{\omega\pm}$ with $\mathtt{g}_{\pm}^{\omega}$ as the coefficients (Noted, $g$, $g$ and $\mathtt{g}$[1] are 3 separate characters employing distinct mathematical fonts, despite their visual resemblance):

$$\bar{g}_{\curlywedge}^{\omega} := \overline{\mathtt{g}_{\pm}^{\omega}}^{\mathsf{T}} \cdot \overline{\bar{g}_{\curlywedge}^{\omega\pm}} := \begin{pmatrix} \mathtt{g}_{+}^{\omega} & \mathtt{g}_{-}^{\omega} \end{pmatrix} \begin{pmatrix} \bar{g}_{\curlywedge}^{\omega+} \\ \bar{g}_{\curlywedge}^{\omega-} \end{pmatrix} = \sum_{\pm} \mathtt{g}_{\pm}^{\omega} \bar{g}_{\curlywedge}^{\omega\pm} =: \sum_{\pm} \bar{\mathtt{g}}_{\curlywedge}^{\omega\pm}, \tag{S50}$$

4 | 26, 26, 27, 28.

where $\mathtt{g}_{\pm}^{\omega}$ denote the undetermined *basis coefficients* or *complex amplitude* for the computable polarization states $\bar{g}_{\curlywedge}^{\omega\pm}$ corresponding to the *overall mode field* $\bar{\mathtt{g}}_{\curlywedge}^{\omega\pm} := \mathtt{g}_{\pm}^{\omega} \bar{g}_{\curlywedge}^{\omega\pm}$, and the values of $\mathtt{g}_{\pm}^{\omega}$ will be determined later by known $\bar{g}_{\curlywedge}^{\omega\pm}$ or $\bar{g}_{\rho}^{\omega\pm}$, which is then determined by the boundary conditions[2] or given directly.

When combined with the *propagating/diffraction/phase part/component/factor* $\mathbb{e}^{\mathbb{i}\bar{k}_{\pm}^{\omega}\cdot\bar{r}}$ determined by the computable eigenvalues $k_{\pm}^{\omega}$, Eq. (S50) forms the traveling wave solution $\bar{G}_{\curlywedge\bar{r}}^{\omega}$ to Eq. (S5b) in the spatiotemporal frequency domain:

$$\bar{G}_{\curlywedge\bar{r}}^{\omega} := \overline{\bar{g}_{\curlywedge}^{\omega\pm}}^{\mathsf{T}} \cdot \overline{\mathbb{e}^{\mathbb{i}\bar{k}_{\pm}^{\omega}\cdot\bar{r}}} := \begin{pmatrix} \bar{g}_{\curlywedge}^{\omega+} & \bar{g}_{\curlywedge}^{\omega-} \end{pmatrix} \begin{pmatrix} \mathbb{e}^{\mathbb{i}\bar{k}_{+}^{\omega}\cdot\bar{r}} \\ \mathbb{e}^{\mathbb{i}\bar{k}_{-}^{\omega}\cdot\bar{r}} \end{pmatrix} = \sum_{\pm} \bar{g}_{\curlywedge}^{\omega\pm} \mathbb{e}^{\mathbb{i}\bar{k}_{\pm}^{\omega}\cdot\bar{r}} =: \sum_{\pm} \bar{G}_{\curlywedge\bar{r}}^{\omega\pm} \tag{S51a}$$

$$= \overline{\bar{g}_{\curlywedge}^{\omega\pm} \mathbb{e}^{\mathbb{i}\bar{k}_{\pm}^{\omega}\cdot\bar{r}}}^{\mathsf{T}} \cdot \overline{\mathtt{g}_{\pm}^{\omega}} = \overline{\bar{g}_{\curlywedge}^{\omega\pm}}^{\mathsf{T}} \cdot \overline{\overline{\mathbb{e}^{\mathbb{i}\bar{k}_{\pm}^{\omega}\cdot\bar{r}}}} \cdot \overline{\mathtt{g}_{\pm}^{\omega}} = \overline{\bar{g}_{\curlywedge}^{\omega\pm}}^{\mathsf{T}} \cdot \overline{\mathtt{g}_{\pm}^{\omega} \mathbb{e}^{\mathbb{i}\bar{k}_{\pm}^{\omega}\cdot\bar{r}}} =: \overline{\bar{g}_{\curlywedge}^{\omega\pm}}^{\mathsf{T}} \cdot \overline{\mathtt{G}_{\bar{r}}^{\omega\pm}}, \tag{S51b}$$

where the propagating part $\overline{\overline{\mathbb{e}^{\mathbb{i}\bar{k}_{\pm}^{\omega}\cdot\bar{r}}}}$ is defined as a diagonal matrix:

$$\overline{\overline{\mathbb{e}^{\mathbb{i}\bar{k}_{\pm}^{\omega}\cdot\bar{r}}}} := \mathrm{diag}\left[\mathbb{e}^{\mathbb{i}\bar{k}_{+}^{\omega}\cdot\bar{r}}, \mathbb{e}^{\mathbb{i}\bar{k}_{-}^{\omega}\cdot\bar{r}}\right] = \begin{pmatrix} \mathbb{e}^{\mathbb{i}\bar{k}_{+}^{\omega}\cdot\bar{r}} & 0 \\ 0 & \mathbb{e}^{\mathbb{i}\bar{k}_{-}^{\omega}\cdot\bar{r}} \end{pmatrix}. \tag{S52}$$

Attention should be given to the fact that the independent variables of the general solution $\bar{g}_{\curlywedge}^{\omega}, \bar{G}_{\curlywedge\bar{r}}^{\omega}$ from Eqs. (S50) and (S51) can be either spherical $\hat{k} \in \mathbb{R}_{\ominus}^{2}$ (related to Eq. (S10)) or Cartesian $\bar{k}_{\rho} \in \mathbb{R}_{\rho}^{2}$ (linked to Eq. (S6)).

The two set of general solutions $\bar{g}_{\curlywedge}^{\omega}(\hat{k}), \bar{G}_{\curlywedge\bar{r}}^{\omega}(\hat{k})$ & $\bar{g}_{\curlywedge}^{\omega}\left(\bar{k}_{\rho}\right), \bar{G}_{\curlywedge\bar{r}}^{\omega}\left(\bar{k}_{\rho}\right)$ with distinct independent variables $\hat{k}, \bar{k}_{\rho}$ carry varied meanings: when $\bar{g}_{\curlywedge}^{\omega}(\hat{k}), \bar{G}_{\curlywedge\bar{r}}^{\omega}(\hat{k})$ are functions of real directions $\hat{k}$ in reciprocal space, the transverse wave vectors $\bar{k}_{\rho}^{\omega}(\hat{k}) = \left[\bar{k}^{\omega}(\hat{k})\right]_{\rho} =$

[1] Noted, even though the symbol $\mathtt{g}$ is in upright/regular font, it still represents a continuous variable, which breaks the preset rule↰ in Section 2 for the first time.

[2] where the most fundamental independent variables of the general solution $\bar{g}_{\curlywedge}^{\omega}$ should share a common $\bar{k}_{\rho} \in \mathbb{R}_{\rho}^{2}$ (rather than $\hat{k} \in \mathbb{R}_{\ominus}^{2}$) grid, in order to be able to integrate back to the total field $\bar{E}_{\rho}^{\omega}$ in real space, to which the boundary conditions are applied.

$\left[k'^{\omega}(\hat{k})\hat{k}\right]_{\rho} \in \mathbb{C}_{\perp}^{2}$ are generally complex, preventing the formation of real spatial frequency grid $\bar{k}_{\rho} \in \mathbb{R}_{\rho}^{2}$, and thus, not aligning with Fourier optics(FO).

The FO framework necessitates selecting real $\bar{k}_{\rho} \in \mathbb{R}_{\rho}^{2}$ for $\bar{g}_{\curlywedge}^{\omega}\left(\bar{k}_{\rho}\right), \bar{G}_{\curlywedge \bar{r}}^{\omega}\left(\bar{k}_{\rho}\right)$ as their independent variables, leading to the occurrence of $\bar{k}^{\omega} \cdot \bar{r} = \bar{k}_{\rho} \cdot \bar{\rho} + k_{z}^{\omega}\left(\bar{k}_{\rho}\right)(z - z_0)$ rather than $\bar{k}^{\omega} \cdot \bar{r} = k'^{\omega}(\hat{k})\hat{k} \cdot \bar{r}$. This naturally causes the separation of the transverse spatial frequency component $\bar{k}_{\rho} \cdot \bar{\rho}$ (or rather, $\mathbb{e}^{\mathbb{i}\bar{k}_{\rho} \cdot \bar{\rho}}$) from the propagating part $\mathbb{e}^{\mathbb{i}\bar{k}_{\pm}^{\omega} \cdot \bar{r}}$ of $\bar{G}_{\curlywedge \bar{r}}^{\omega}$ in Eq. (S51), and ultimately results in the general solution for the spatiotemporal spectrum of the electric field $\bar{G}_{\curlywedge z}^{\omega} = \bar{G}_{\curlywedge \bar{r}}^{\omega} / \mathbb{e}^{\mathbb{i}\bar{k}_{\rho} \cdot \bar{\rho}}$:

$$\bar{G}_{\curlywedge z}^{\omega} := \overline{\bar{g}_{\curlywedge}^{\omega\pm}}^{\mathsf{T}} \cdot \overline{\mathbb{e}^{\mathbb{i}k_{z}^{\omega\pm}(z-z_0)}} = \sum_{\pm} \bar{g}_{\curlywedge}^{\omega\pm} \mathbb{e}^{\mathbb{i}k_{z}^{\omega\pm}(z-z_0)} =: \sum_{\pm} \bar{G}_{\curlywedge z}^{\omega\pm} \tag{S53a}$$

$$= \overline{\bar{g}_{\curlywedge}^{\omega\pm}}^{\mathsf{T}} \cdot \overline{\overline{\mathbb{e}^{\mathbb{i}k_{z}^{\omega\pm}(z-z_0)}}} \cdot \overline{\mathtt{g}_{\pm}^{\omega}} \xrightarrow{\mathtt{G}_{z_0} := \mathtt{g}} \overline{\bar{g}_{\curlywedge}^{\omega\pm}}^{\mathsf{T}} \cdot \overline{\mathtt{g}_{\pm}^{\omega} \mathbb{e}^{\mathbb{i}k_{z}^{\omega\pm}(z-z_0)}} =: \overline{\bar{g}_{\curlywedge}^{\omega\pm}}^{\mathsf{T}} \cdot \overline{\mathtt{G}_{z}^{\omega\pm}}, \tag{S53b}$$ *3* | *27*, *28*, *28*.

wherein the diagonal matrix $\overline{\overline{\mathbb{e}^{\mathbb{i}k_{z}^{\omega\pm}(z-z_0)}}}$ is typically called the *propagation matrix*:

$$\overline{\overline{\mathbb{e}^{\mathbb{i}k_{z}^{\omega\pm}(z-z_0)}}} := \mathrm{diag}\left[\mathbb{e}^{\mathbb{i}k_{z}^{\omega+}(z-z_0)}, \mathbb{e}^{\mathbb{i}k_{z}^{\omega-}(z-z_0)}\right] = \begin{pmatrix} \mathbb{e}^{\mathbb{i}k_{z}^{\omega+}(z-z_0)} & 0 \\ 0 & \mathbb{e}^{\mathbb{i}k_{z}^{\omega-}(z-z_0)} \end{pmatrix}, \tag{S54}$$ *1* | *28*.

and we have implicitly defined:

$$\text{overall vector field} \quad \bar{G}_{\curlywedge z_0}^{\omega} := \bar{g}_{\curlywedge}^{\omega}, \tag{S55a}$$

$$\text{polarization states / bases} \quad \bar{G}_{\curlywedge z}^{\omega\pm} \equiv \bar{g}_{\curlywedge}^{\omega\pm}, \tag{S55b}$$

$$\text{complex amplitudes / basis coefficients} \quad \mathtt{G}_{z_0}^{\omega\pm} := \mathtt{g}_{\pm}^{\omega}. \tag{S55c}$$

We now initiate the consideration of the transition matrix connecting two cross-sections at $z_0, z$ $(0 < z_0, z < L)$ within the slab material for the general spatiotemporal spectrum solution of the electric field $\bar{G}_{\curlywedge z}^{\omega}$.

The eigensystem $k_{z}^{\omega\pm}, \bar{g}_{\curlywedge}^{\omega\pm}$ of the wave Eq. (S6) is determined (see Figs. S4 to S6) for a specific slab material $\underline{\bar{u}}^{\omega}, \underline{\bar{\alpha}}^{\omega}$ and a given $\mathcal{C}$ frame orientation $\underline{\bar{O}_{\mathcal{C}}}$, leading to the determination of the first two matrices in $\bar{G}_{\curlywedge z}^{\omega} = \overline{\bar{g}_{\curlywedge}^{\omega\pm}}^{\mathsf{T}} \cdot \overline{\overline{\mathbb{e}^{\mathbb{i}k_{z}^{\omega\pm}(z-z_0)}}} \cdot \overline{\mathtt{g}_{\pm}^{\omega}}$ from Eq. (S53b), namely the polarization matrix $\overline{\bar{g}_{\curlywedge}^{\omega\pm}}^{\mathsf{T}}$ formed by paired eigenvectors $\bar{g}_{\curlywedge}^{\omega\pm}$ (2 polarization states), along with the propagation matrix $\overline{\overline{\mathbb{e}^{\mathbb{i}k_{z}^{\omega\pm}(z-z_0)}}}$ composed of paired eigenvalues $k_{z}^{\omega\pm}$ (related to 2 refractive indices $n'^{\omega}_{\pm}$). The only remaining task is to ascertain the last column vector $\overline{\mathtt{g}_{\pm}^{\omega}}$ constructed from paired basis coefficients $\mathtt{g}_{\pm}^{\omega}$ (2 complex amplitudes).

Basis coefficients $\mathtt{g}_{\pm}^{\omega}$ are solely determined by boundary conditions and remain constant during propagation, similar to the $z$-independence of polarization states $\bar{g}_{\curlywedge}^{\omega\pm}$. However, one can determine the values of basis coefficients $\mathtt{g}_{\pm}^{\omega}$ by simply knowing the transverse part $\bar{G}_{\rho z_0}^{\omega} = \bar{g}_{\rho}^{\omega} = \left(g_{x}^{\omega}, g_{y}^{\omega}\right)^{\mathsf{T}} = \overline{\mathtt{g}_{\pm}^{\omega}}^{\mathsf{T}} \cdot \overline{\bar{g}_{\rho}^{\omega\pm}}$ of $\bar{g}_{\curlywedge}^{\omega}$ from Eq. (S50), or $\bar{G}_{\curlywedge z_0}^{\omega}$ from Eq. (S53) on any specific cross-section at $z_0$ within the crystal. This means that, although determined by boundary conditions, basis coefficient $\mathtt{g}_{\pm}^{\omega}$ and the

column vector $\overline{\mathsf{g}^{\omega}_{\pm}}$ built from it can be established through alternative information, and remains fixed once known.

Extracting the transverse ($[\cdot]_{\rho} = \mathcal{T}_{xy}[\cdot]$) component $\left(G^{\omega}_{xz_0},\ G^{\omega}_{yz_0}\right)^{\intercal} = \bar{G}^{\omega}_{\rho z_0} = \overline{\bar{g}^{\omega\pm}_{\rho}}^{\intercal} \cdot \overline{\mathsf{g}^{\omega}_{\pm}}$ of $\bar{G}^{\omega}_{\lambda z}$ in Eq. (S53b) at $z = z_0$, and left-multiplying it by $\overline{\bar{g}^{\omega\pm}_{\rho}}^{-\intercal} := \left[\overline{\bar{g}^{\omega\pm}_{\rho}}^{\intercal}\right]^{-1}$ leads to the *basis-coefficients column vector*

$$\overline{\mathsf{g}^{\omega}_{\pm}} = \overline{\bar{g}^{\omega\pm}_{\rho}}^{-\intercal} \cdot \bar{G}^{\omega}_{\rho z_0}, \tag{S56}$$ *1* | *28.*

which is then inserted into Eq. (S53b) to acquire the $3 \times 2$ transition matrix $\bar{\bar{T}}^{\omega}_{\lambda z\rho}$[1] that transforms $\bar{G}^{\omega}_{\rho z_0} \to \bar{G}^{\omega}_{\lambda z}$:

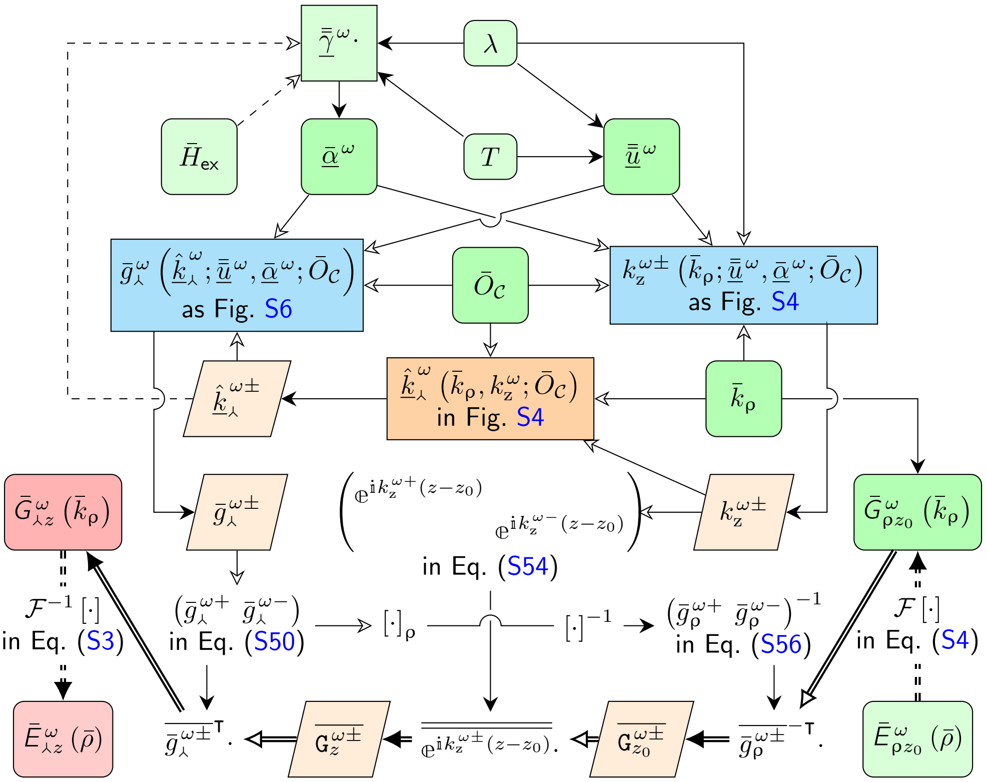


Quoted @ *9* pp. *23*, *23*, *24*, *25*, *29*, *29*, *29*, *29*, *30*.

**Fig. S7** Flowchart for Accessing $\bar{G}^{\omega}_{\lambda z}\left(\bar{k}_{\rho};\underline{\bar{u}}^{\omega},\underline{\bar{\alpha}}^{\omega};\bar{O}_{\mathcal{C}};\bar{G}^{\omega}_{\rho z_0}\right)$ as the output of Eq. (S57) — the built-from-source white box solver for $\bar{G}^{\omega}_{\rho z_0}\left(\bar{k}_{\rho}\right) \to \bar{G}^{\omega}_{\lambda z}\left(\bar{k}_{\rho}\right)$ transition, together with the corresponding $\bar{E}^{\omega}_{\rho z_0}(\bar{\rho}) \to \bar{E}^{\omega}_{\lambda z}(\bar{\rho})$ mapping chain as the core algorithm and main result of this paper. All functions presented in Figs. S1, S2, S3, S4, S5 and S6 were invoked by this flowchart. For the meanings of styles of nodes & arrows, see Tables S1 and S2.

[1] which outwardly looks similar to the $3 \times 2$ transformation matrix $\bar{\bar{\mathcal{T}}}_{\lambda\Theta}$ from Eq. (S30)

$$\bar{G}^{\omega}_{\text{⅄}z} = \bar{\bar{T}}^{\omega}_{\text{⅄}z\rho} \cdot \bar{G}^{\omega}_{\rho z_0} \tag{S57a}$$

$$= \overline{g^{\omega\pm}_{\text{⅄}}}^{\mathsf{T}} \cdot \overline{\overline{\mathbb{e}^{\mathbb{i}k_z^{\omega\pm}(z-z_0)}}} \cdot \overline{g^{\omega\pm}_{\rho}}^{-\mathsf{T}} \cdot \bar{G}^{\omega}_{\rho z_0}. \tag{S57b}$$

As the pivotal formula throughout this article, the Eq. (S57) above outlines the forward diffraction process of electromagnetic field's $\mathrm{x, y, z}$ components within homogeneous materials possessing arbitrary $\bar{\bar{\varepsilon}}$. This encompasses low/high-order isotropic/anisotropic linear/circular diffraction/absorption/gain, cross-coupling between $\mathrm{x, y, z}$ components, lateral/longitudinal *spin-orbit interaction* (SOI)[69] and other related processes, essentially covering most aspects of linear crystal optics(LCO).

The mapping described by Eq. (S57) transforms a 2-component column vector $\bar{G}^{\omega}_{\rho z_0}$ into a 3-component $\bar{G}^{\omega}_{\text{⅄}z}$, introducing redundant information in the output $\bar{G}^{\omega}_{\text{⅄}z}$ relative to the input $\bar{G}^{\omega}_{\rho z_0}$. This redundancy is attributed to the transverse nature of optical/electromagnetic waves.

As the principal outcome of this paper, the $3 \times 2$ transition matrix $\bar{\bar{T}}^{\omega}_{\text{⅄}z\rho} = \overline{g^{\omega\pm}_{\text{⅄}}}^{\mathsf{T}} \cdot \overline{\overline{\mathbb{e}^{\mathbb{i}k_z^{\omega\pm}(z-z_0)}}} \cdot \overline{g^{\omega\pm}_{\rho}}^{-\mathsf{T}}$ presented in Eq. (S57) can be depicted as a flowchart in Fig. S7. This chart comprehensively details all macro and micro processes starting from the base-level input variables (original specific parameters) to the top-level cumulative matrix/tensor fields (ultimate abstract operators), along with the deeply wrapped internal call-stack structure of the main function.

From a programmatic perspective, the following Tables S1 and S2 illustrate the meaning of each element (node or arrow) in Figs. S1 to S7.

Quoted @ *8* pp. *16*, *16*, *22*, *23*, *24*, *25*, *28*, *29*.

**Table S1** The definitions of styles of nodes within Figs. S1, S2, S3, S4, S5, S6 and S7.

| | | | | |
|---|---|---|---|---|
| Intermediate | `Node: Switch Flow` | ◇ | conditionally in a flowchart as | *if* |
| Initial void | `Node: Main Origin` | ▢ (yellow) | at the start of a flowchart as its | *entry* |
| Intermediate | `Data: Private Var` | ▱ | can't be used by other flowcharts | |
| Intermediate | `Data: Public Var` | ▱ (orange) | may be used by other flowcharts as | ▢ / □ |
| Initial input | `Data: Parameter` | ▢ (green) | at the start of a flowchart as its | **args* |
| Initial input | `Data: Parameter` | ▢ (orange) | from within another flowchart as its | ▱ |
| Final output | `Data: Result` | ▢ | at the end of a flowchart as its | *return* |
| Intermediate | `Function/Operator` | □ (white) | from (within) / as an equation | |
| Intermediate | `Function/Operator` | □ (blue) | from / as another flowchart as its | ▢(·) |
| Intermediate | `Function/Operator` | □ (orange) | from within another flowchart as its | ▱(·) |

Quoted @ *8* pp. *16*, *16*, *22*, *23*, *24*, *25*, *28*, *29*.

**Table S2** The meanings of styles of arrows within Figs. S1, S2, S3, S4, S5, S6 and S7.

| | | | |
|---|---|---|---|
| Main streams<br>Side streams | ⟹▷ and = =▷<br>⟶▷ and - - ▷ | all equal to | `Data` as the input of `Operator` |
| Main streams<br>Side streams | ⟹▶ and = =▶<br>⟶➤ and - - ➤ | all equal to | `Operator` returns its output of `Data`<br>or: `Data` as a `Function` of `Data`<br>or: `Operator` as a `Function` of `Operator` |

When materials exhibit absorption or gain (displaying linear and/or circular dichroism), both $\bar{\bar{\varepsilon}}_{\mathrm{r}}^{\prime\omega}, \bar{\bar{\eta}}^{\omega}$ from Eq. (S31) and the corresponding characteristic matrix $\underline{\bar{\bar{m}}}_{\theta\phi}^{\prime\omega}$ from Eq. (S40) are real/complex non-Hermitian. Then the corresponding two eigenvalues $k_{\mathrm{z}}^{\omega\pm}$ are complex (having non-zero imaginary parts), and the corresponding two eigenvectors $\bar{g}_{\lambda}^{\omega\pm}$ in Eq. (S48) (or $\bar{d}_{\lambda}^{\omega\pm}$) are complex non-orthogonal, which suggests that (the transverse part $\overline{\bar{g}_{\rho}^{\omega\pm}}^{\mathsf{T}}$ of) the $3 \times 2$ polarization matrix $\overline{\bar{g}_{\lambda}^{\omega\pm}}^{\mathsf{T}}$ in Eq. (S57) and Fig. S7 formed by these paired 3-component eigenvectors $\bar{g}_{\lambda}^{\omega\pm}$ are non-unitary.

# References


Cited @ 14 pp. 3, 4, 4, 5, 5, 6, 6, 7, 10, 11, 11, 12, 18, 23.

[1] McLeod, R. R. & Wagner, K. H. Vector Fourier optics of anisotropic materials **6**, 368. URL https://opg.optica.org/aop/abstract.cfm?uri=aop-6-4-368.

[2] Zhang, S. & Wyrowski, F. Wyrowski, F., Sheridan, J. T. & Meuret, Y. (eds) *Fully vectorial simulation of light propagation through uniaxial and biaxial crystals.* (eds Wyrowski, F., Sheridan, J. T. & Meuret, Y.) , 988909. URL http://proceedings.spiedigitallibrary.org/proceeding.aspx?doi=10.1117/12.2234310.

Cited @ 1 p. 3.

Cited @ 4 pp. 3, 4, 6, 6.

[3] Zarifi, D., Soleimani, M. & Abdolali, A. Plane Wave Reflection and Transmission from Uni- and Bi- Axial Chiral Slabs **10**.

[4] Berreman, D. W. Optics in Stratified and Anisotropic Media: 4×4-Matrix Formulation **62**, 502. URL https://opg.optica.org/abstract.cfm?URI=josa-62-4-502.

Cited @ 8 pp. 3, 3, 4, 4, 4, 6, 6, 6.

Cited @ 6 pp. 3, 4, 4, 5, 6, 6.

[5] Abdulhalim, I. Exact 2 × 2 matrix method for the transmission and reflection at the interface between two arbitrarily oriented biaxial crystals **1**, 655–661. URL https://iopscience.iop.org/article/10.1088/1464-4258/1/6/301.

[6] Olyslager, F. & Lindell, I. Electromagnetics and exotic media: A quest for the holy grail **44**, 48–58. URL http://ieeexplore.ieee.org/document/1003634/.

Cited @ 1 p. 3.

Cited @ 12 pp. 3, 4, 4, 5, 5, 5, 6, 6, 6, 6, 7, 11.

[7] Chang, P.-H., Kuo, C.-Y. & Chern, R.-L. Wave propagation in bianisotropic metamaterials: Angular selective transmission .

[8] Zhao, X. *et al.* Nontrivial phase matching in helielectric polarization helices: Universal phase matching theory, validation, and electric switching **119**, e2205636119. URL https://pnas.org/doi/full/10.1073/pnas.2205636119.

Cited @ 1 p. 3.

Cited @ 10 pp. 3, 5, 5, 6, 7, 14, 18, 18, 18, 19.

[9] Zu, R. *et al.* Analytical and numerical modeling of optical second harmonic generation in anisotropic crystals using ♯SHAARP package **8**, 246. URL https://www.nature.com/articles/s41524-022-00930-4.

[10] Stallinga, S. Berreman 4×4 matrix method for reflective liquid crystal displays **85**, 3023–3031. URL https://pubs.aip.org/jap/article/85/6/3023/178429/Berreman-4-4-matrix-method-for-reflective-liquid.

Cited @ 9 pp. 4, 4, 4, 5, 6, 6, 6, 6, 6.

Cited @ 5 pp. 4, 6, 6, 6, 6.

[11] Moler, C. & Van Loan, C. Nineteen dubious ways to compute the exponential of a matrix, twenty-five years later **45**, 3–49. URL http://epubs.siam.org/doi/10.1137/S00361445024180.

[12] Grundmann, M. & Sturm, C. The singular optical axes in biaxial crystals and analysis of their spectral dispersion effects in $\beta$-ga$_2$O$_3$ **93**, 053839. URL http://arxiv.org/abs/1601.03760.

Cited @ 5 pp. 4, 5, 5, 6, 7.

Cited @ 25 pp. 4, 5, 5, 5, 5, 5, 6, 6, 7, 7, 7, 9, 10, 10, 14, 17, 17, 17, 18, 18, 18, 19, 19, 21, 23.

[13] Berry, M. V. & Dennis, M. R. The optical singularities of birefringent dichroic chiral crystals **459**, 1261–1292. URL https://royalsocietypublishing.org/doi/10.

1098/rspa.2003.1155.

[14] Berry, M. The optical singularities of bianisotropic crystals **461**, 2071–2098. URL https://royalsocietypublishing.org/doi/10.1098/rspa.2005.1507.
Cited @ *16* pp. *4*, *5*, *5*, *5*, *5*, *5*, *5*, *6*, *6*, *6*, *6*, *6*, *7*, *7*, *7*, *20*.

Cited @ *2* pp. *4*, *4*.
[15] Mackay, T. G., Zhou, C. & Lakhtakia, A. *Exceptional guided waves*, 1–4. URL https://ieeexplore.ieee.org/document/9560546.

[16] Yang, Y. *et al.* Non-abelian physics in light and sound **383**, eadf9621. URL https://www.science.org/doi/10.1126/science.adf9621.
Cited @ *1* p. *4*.

Cited @ *6* pp. *4*, *4*, *4*, *4*, *6*, *6*.
[17] Borzdov, G. N. Waves with linear, quadratic and cubic coordinate dependence of amplitude in crystals **46**, 245–257. URL http://link.springer.com/10.1007/BF02846911.

[18] Sturm, C. Electromagnetic waves in crystals: The presence of exceptional points **5**, 2300235. URL https://onlinelibrary.wiley.com/doi/abs/10.1002/adpr.202300235.
Cited @ *12* pp. *4*, *4*, *4*, *4*, *4*, *4*, *5*, *5*, *6*, *6*, *6*, *7*.

Cited @ *1* p. *4*.
[19] Berry, M. Pancharatnam, virtuoso of the poincaré sphere: An appreciation **67**, 220–223. URL https://www.jstor.org/stable/24095727.

[20] Gerardin, J. & Lakhtakia, A. Conditions for Voigt wave propagation in linear, homogeneous, dielectric mediums **112**, 493–495. URL https://linkinghub.elsevier.com/retrieve/pii/S0030402604700807.
Cited @ *5* pp. *4*, *4*, *5*, *6*, *7*.

Cited @ *6* pp. *4*, *5*, *7*, *7*, *18*, *22*.
[21] Ossikovski, R., Arteaga, O. & Sturm, C. Constitutive relations for optically active anisotropic media: A review **2**, 2100160. URL https://onlinelibrary.wiley.com/doi/10.1002/adpr.202100160.

[22] Ossikovski, R. & Arteaga, O. Extended yeh's method for optically active anisotropic layered media **42**, 3690. URL https://opg.optica.org/abstract.cfm?URI=ol-42-18-3690.
Cited @ *8* pp. *4*, *5*, *6*, *6*, *7*, *18*, *18*, *22*.

Cited @ *5* pp. *4*, *5*, *6*, *6*, *6*.
[23] Yeh, P. Electromagnetic propagation in birefringent layered media .

[24] Chern, R.-L. & Yu, Y.-Z. Chiral surface waves on hyperbolic-gyromagnetic metamaterials .
Cited @ *5* pp. *4*, *5*, *6*, *10*, *11*.

Cited @ *2* pp. *4*, *18*.
[25] Grundmann, M. *et al.* Optically anisotropic media: New approaches to the dielectric function, singular axes, microcavity modes and Raman scattering intensities **11**, 1600295. URL https://onlinelibrary.wiley.com/doi/10.1002/pssr.201600295.

[26] Zhang, S., Asoubar, D. & Wyrowski, F. Glebov, A. L. & Leisher, P. O. (eds) *Rigorous modeling of laser light propagation through uniaxial and biaxial crystals.* (eds Glebov, A. L. & Leisher, P. O.) , 93460N. URL http://proceedings.spiedigitallibrary.org/proceeding.aspx?doi=10.1117/12.2079534.
Cited @ *1* p. *5*.

Cited @ *4* pp. *5*, *5*, *6*, *7*.
[27] Chen, H. C. A coordinate-free approach to wave propagation in anisotropic media

**53**, 4606–4609. URL http://aip.scitation.org/doi/10.1063/1.331382.

[28] Asoubar, D., Zhang, S. & Wyrowski, F. Simulation of birefringence effects on the dominant transversal laser resonator mode caused by anisotropic crystals **23**, 13848. URL https://opg.optica.org/abstract.cfm?URI=oe-23-11-13848. Cited @ *4* pp. *5*, *5*, *6*, *6*.

Cited @ *3* pp. *5*, *6*, *7*. [29] Kirillov, O., Mailybaev, A. & Seyranian, A. *On eigenvalue surfaces near a diabolic point*, 319–325 (IEEE). URL http://ieeexplore.ieee.org/document/1514000/.

[30] Mackay, T. G. & Lakhtakia, A. *Electromagnetic Anisotropy and Bianisotropy: A Field Guide* 2 edn (WORLD SCIENTIFIC). URL https://www.worldscientific.com/worldscibooks/10.1142/11351. Cited @ *6* pp. *5*, *5*, *6*, *7*, *8*, *18*.

Cited @ *8* pp. *5*, *5*, *6*, *7*, *10*, *10*, *18*, *18*. [31] Brenier, A. Lasing with conical diffraction feature in the KGd(WO4)2:Nd biaxial crystal **122**, 237. URL http://link.springer.com/10.1007/s00340-016-6512-y.

[32] Chang, P. C., Walker, J. & Hopcraft, K. Ray tracing in absorbing media **96**, 327–341. URL https://linkinghub.elsevier.com/retrieve/pii/S002240730500066X. Cited @ *5* pp. *5*, *5*, *7*, *11*, *12*.

Cited @ *4* pp. *5*, *5*, *7*, *19*. [33] Wang, Y., Liang, L., Xin, H. & Wu, L. Complex ray tracing in uniaxial absorbing media **25**, 653. URL https://opg.optica.org/abstract.cfm?URI=josaa-25-3-653.

[34] Dupertuis, M. A. & Proctor, M. Generalization of complex Snell-Descartes and Fresnel laws . Cited @ *1* p. *5*.

Cited @ *4* pp. *5*, *5*, *6*, *7*. [35] Chang, C.-M. & Shieh, H.-P. D. Simple Formulas for Calculating Wave Propagation and Splitting in Anisotropic Media **40**, 6391. URL https://iopscience.iop.org/article/10.1143/JJAP.40.6391.

[36] Wang, Y., Shi, P., Xin, H. & Wu, L. Complex ray tracing in biaxial anisotropic absorbing media **10**, 075009. URL https://iopscience.iop.org/article/10.1088/1464-4258/10/7/075009. Cited @ *2* pp. *5*, *19*.

Cited @ *3* pp. *5*, *6*, *6*. [37] Chen, H. C. A coordinate-free approach to wave reflection from an anisotropic medium **16**, 1213–1215. URL http://doi.wiley.com/10.1029/RS016i006p01213.

[38] Chen, H. C. *Theory of Electromagnetic Waves: A Coordinate-Free Approach* McGraw-Hill Series in Electrical Engineering (McGraw-Hill Book Co). Cited @ *3* pp. *5*, *6*, *6*.

Cited @ *3* pp. *5*, *6*, *6*. [39] Budden, K. G. *The Propagation of Radio Waves: The Theory of Radio Waves of Low Power in the Ionosphere and Magnetosphere* (Cambridge University Press). URL https://www.cambridge.org/core/books/propagation-of-radio-waves/BD8F03DDFEC9E2D3ABB1CAD7DEF3B91A.

[40] Dmitriev, V. G. Effective nonlinearity coefficients for three-wave interactions in biaxial crystals of mm2 point group symmetry . Cited @ *3* pp. *7*, *18*, *18*.

Cited @ *8* pp. *7*, *14*, *18*, *18*, *18*, *18*, *18*, *19*.

[41] Diesperov, K. V. & Dmitriev, V. G. Effective nonlinear coefficient for sum-frequency generation with collinear phase matching calculated taking account of the birefringence in biaxial crystals **27**, 433–436. URL https://iopscience.iop.org/article/10.1070/QE1997v027n05ABEH000966.

[42] Mackay, T. G. & Lakhtakia, A. Exorcizing ghost waves **192**, 162926. URL https://linkinghub.elsevier.com/retrieve/pii/S0030402619308034.

Cited @ *1* p. *8*.

Cited @ *1* p. *11*.

[43] Grechin, S. G., Nikolaev, P. P. & Okhrimchuk, A. G. Fourier space method for calculating the propagation of laser radiation in biaxial crystals taking into account the angle between the eigenpolarisations **44**, 34–41. URL http://stacks.iop.org/1063-7818/44/i=1/a=34?key=crossref.c0a29a2463a78f48c3bee05f372ac044.

[44] Waseer, W. I., Naqvi, Q. A. & Mughal, M. J. Non-uniform plane waves (ghost waves) in general anisotropic medium **453**, 124334. URL https://linkinghub.elsevier.com/retrieve/pii/S0030401819306790.

Cited @ *1* p. *11*.

Cited @ *3* pp. *11*, *17*, *18*.

[45] Kuznetsov, E. V. & Merzlikin, A. M. Conical refraction in a magneto-optical biaxial crystal **19**, 055610. URL https://iopscience.iop.org/article/10.1088/2040-8986/aa663e.

[46] Landau, L. D. & Lifshitz, E. M. in *CHAPTER XI - ELECTROMAGNETIC WAVES IN ANISOTROPIC MEDIA* (eds Landau, L. D. & Lifshitz, E. M.) *Electrodynamics of Continuous Media (Second Edition)*, Vol. 8 of *Course of Theoretical Physics* 331–357 (Pergamon).

Cited @ *9* pp. *11*, *14*, *17*, *17*, *17*, *17*, *17*, *17*, *18*.

Cited @ *4* pp. *14*, *18*, *18*, *18*.

[47] Nye, J. F. *Physical Properties of Crystals: Their Representation by Tensors and Matrices* Reprinted edn. Oxford Science Publications (Clarendon Press).

[48] Schell, A. J. & Bloembergen, N. Laser studies of internal conical diffraction II Intensity patterns in an optically active crystal, $\alpha$-iodic acid* **68**, 1098. URL https://opg.optica.org/abstract.cfm?URI=josa-68-8-1098.

Cited @ *3* pp. *17*, *18*, *18*.

Cited @ *2* pp. *17*, *18*.

[49] Kuznetsov, E. V. & Merzlikin, A. M. Light propagation in a magneto-optical hyperbolic biaxial crystal **405**, 164–170. URL https://linkinghub.elsevier.com/retrieve/pii/S0030401817307010.

[50] Nelson, D. F. Mechanisms and dispersion of crystalline optical activity **6**, 1110–1116. URL https://opg.optica.org/josab/abstract.cfm?uri=josab-6-6-1110.

Cited @ *1* p. *18*.

Cited @ *1* p. *18*.

[51] Nelson, D. F. Deriving the transmission and reflection coefficients of an optically active medium without using boundary conditions **51**, 6142–6153. URL https://link.aps.org/doi/10.1103/PhysRevE.51.6142.

[52] Brenier, A., Majchrowski, A. & Michalski, E. Chirality versus dichroism: Competition and role in conical diffraction displayed from the Nd:Bi2ZnOB2O6 acentric biaxial laser crystal **72**, 813–820. URL https://linkinghub.elsevier.com/retrieve/

Cited @ *2* pp. *18*, *18*.

pii/S0925346717304809.

Cited @ *1* p. *18*. [53] Belsky, A. & Stepanov, M. Internal conical refraction of light beams in biaxial gyrotropic crystals **204**, 1–6. URL https://linkinghub.elsevier.com/retrieve/pii/S0030401802011914.

[54] Eimerl, D. Quantum electrodynamics of optical activity in birefringent crystals **5**, 1453. URL https://opg.optica.org/abstract.cfm?URI=josab-5-7-1453. Cited @ *1* p. *18*.

Cited @ *1* p. *18*. [55] Franta, D. & Vohánka, J. r. Constitutive equations describing optical activity in theory of dispersion **38**, 553–561. URL https://opg.optica.org/josab/abstract.cfm?uri=josab-38-2-553.

[56] Sturm, C., Zviagin, V. & Grundmann, M. Applicability of the constitutive equations for the determination of the material properties of optically active materials **44**, 1351–1354. URL https://opg.optica.org/ol/abstract.cfm?uri=ol-44-6-1351. Cited @ *1* p. *18*.

Cited @ *1* p. *18*. [57] Berry, M. V. & Jeffrey, M. R. Conical diffraction complexified: Dichroism and the transition to double refraction **8**, 1043–1051. URL https://iopscience.iop.org/article/10.1088/1464-4258/8/12/003.

[58] Kato, K. Temperature-tuned 90° phase-matching properties of LiB/sub 3/O/sub 5/ **30**, 2950–2952. URL http://ieeexplore.ieee.org/document/362711/. Cited @ *1* p. *18*.

Cited @ *1* p. *18*. [59] Kato, K. & Takaoka, E. Sellmeier and thermo-optic dispersion formulas for KTP **41**, 5040. URL https://opg.optica.org/abstract.cfm?URI=ao-41-24-5040.

[60] Li, F., Hou, X., Pan, S. & Wang, X. Growth, Structure, and Optical Properties of a Congruent Melting Oxyborate, $Bi_2ZnOB_2O_6$ **21**, 2846–2850. URL https://pubs.acs.org/doi/10.1021/cm900560x. Cited @ *1* p. *18*.

Cited @ *1* p. *18*. [61] Brenier, A. Voigt wave investigation in the $KGd(WO_4)_2$:Nd biaxial laser crystal **17**, 075603. URL https://iopscience.iop.org/article/10.1088/2040-8978/17/7/075603.

[62] Yao, J. Q. & Fahlen, T. S. Calculations of optimum phase match parameters for the biaxial crystal $KTiOPO_4$ **55**, 65–68. URL http://aip.scitation.org/doi/10.1063/1.332850. Cited @ *1* p. *18*.

Cited @ *1* p. *18*. [63] Kaschke, M. & Koch, C. Calculation of nonlinear optical polarization and phase matching in biaxial crystals **49**, 419–423. URL http://link.springer.com/10.1007/BF00325343.

[64] Kholkin, A. L., Pertsev, N. A. & Goltsev, A. V. Piezoelectricity and Crystal Symmetry . Cited @ *1* p. *18*.

Cited @ *1* p. *18*. [65] Boyd, R. W. *Nonlinear Optics* 4 edn (Academic Press is an imprint of Elsevier).

[66] Midwinter, J. E. & Warner, J. The effects of phase matching method and of uniaxial crystal symmetry on the polar distribution of second-order non-linear optical polarization **16**, 1135–1142. URL https://iopscience.iop.org/article/10.1088/0508-3443/16/8/312. Cited @ *1* p. *18*.

Cited @ *1* p. *18*. [67] Yao, J., Shi, W. & Sheng, W. Accurate calculation of the optimum phase-matching parameters in three-wave interactions with biaxial nonlinear-optical crystals **9**, 891. URL https://opg.optica.org/abstract.cfm?URI=josab-9-6-891.

[68] Zhang, S., Partanen, H., Hellmann, C. & Wyrowski, F. Non-paraxial idealized polarizer model **26**, 9840. URL https://opg.optica.org/abstract.cfm?URI=oe-26-8-9840. Cited @ *1* p. *25*.

Cited @ *1* p. *29*. [69] Tang, Y. *et al.* Harmonic spin–orbit angular momentum cascade in nonlinear optical crystals URL http://www.nature.com/articles/s41566-020-0691-0.
